# Supplementary material for: The role of electron correlations in the electronic structure of putative Chern magnet TbMn$_6$Sn$_6$
Source: arXiv:2302.01903 ancillary file (2023-09-28)
Supplement: Supplementary file 1 [file TbMn6Sn6_Supplementary_Information.pdf]

# Supplementary information for “The role of electron correlations in the electronic structure of putative Chern magnet TbMn<sub>6</sub>Sn<sub>6</sub>”

Abdulgani Annaberdiyev,<sup>1</sup> Subhasish Mandal,<sup>2</sup> Lubos Mitas,<sup>3</sup> Jaron T. Krogel,<sup>4</sup> and Panchapakesan Ganesh<sup>5</sup>

<sup>1</sup>Center for Nanophase Materials Sciences, Oak Ridge National Laboratory, Oak Ridge, Tennessee 37831, USA\*

<sup>2</sup>Department of Physics and Astronomy, West Virginia University, Morgantown, WV 26506, USA†

<sup>3</sup>Department of Physics, North Carolina State University, Raleigh, North Carolina 27695-8202, USA

<sup>4</sup>Materials Science and Technology Division, Oak Ridge National Laboratory, Oak Ridge, Tennessee 37831, USA

<sup>5</sup>Center for Nanophase Materials Sciences, Oak Ridge National Laboratory, Oak Ridge, Tennessee 37831, USA ‡

## SUPPLEMENTARY NOTE 1. BULK AND SLAB GEOMETRIES

Throughout this work, we use the experimental geometry from a neutron diffraction study [1]. The structure is reproduced here in Supplementary Table 1. In addition, the structure is also provided in XSF format in Supplementary Table 2.

Supplementary Table 1: Experimental bulk geometry of TbMn<sub>6</sub>Sn<sub>6</sub> [1].  $a = 5.530(1)$  Å,  $c = 9.023(2)$  Å.

| Atom            | Position | Symmetry    | $x$ | $y$ | $z$       |
|-----------------|----------|-------------|-----|-----|-----------|
| Tb              | 1(b)     | $6/mmm$     | 0   | 0   | 1/2       |
| Mn              | 6(i)     | $mm$        | 1/2 | 0   | 0.2525(2) |
| Sn <sub>1</sub> | 2(e)     | $6mm$       | 0   | 0   | 0.1624(1) |
| Sn <sub>2</sub> | 2(d)     | $\bar{6}2m$ | 1/3 | 2/3 | 1/2       |
| Sn <sub>3</sub> | 2(c)     | $\bar{6}2m$ | 1/3 | 2/3 | 0         |

Supplementary Table 2: Experimental bulk geometry of TbMn<sub>6</sub>Sn<sub>6</sub> in XSF format (Angstrom units).

| CRYSTAL      |               |               |               |
|--------------|---------------|---------------|---------------|
| PRIMVEC      |               |               |               |
| 4.7891204829 | -2.7650000000 | 0.0000000000  |               |
| 0.0000000000 | 5.5300000000  | 0.0000000000  |               |
| 0.0000000000 | 0.0000000000  | 9.0230000000  |               |
| PRIMCOORD    |               |               |               |
| 13 1         |               |               |               |
| 65           | 0.0000000000  | 0.0000000000  | -4.5115000000 |
| 25           | 2.3945602415  | 1.3825000000  | 2.2783075000  |
| 25           | -2.3945602415 | 1.3825000000  | 2.2783075000  |
| 25           | 0.0000000000  | -2.7650000000 | 2.2783075000  |
| 25           | 2.3945602415  | 1.3825000000  | -2.2783075000 |
| 25           | -2.3945602415 | 1.3825000000  | -2.2783075000 |
| 25           | -0.0000000000 | -2.7650000000 | -2.2783075000 |
| 50           | 0.0000000000  | 0.0000000000  | 1.4653352000  |
| 50           | -3.1927469886 | -0.0000000000 | -4.5115000000 |
| 50           | -3.1927469886 | -0.0000000000 | 0.0000000000  |
| 50           | 0.0000000000  | 0.0000000000  | -1.4653352000 |
| 50           | -1.5963734943 | 2.7650000000  | 4.5115000000  |
| 50           | -1.5963734943 | 2.7650000000  | 0.0000000000  |

The slab calculation geometries were adapted from the bulk experimental geometry by appropriately terminating it with the Mn surface. We explored the geometry relaxation of the Mn layer as a function of its distance  $z$  to the slab and found no energy gains when  $z$  was incremented by 0.01 Angstroms until  $\Delta z = 0.45$  Angstroms. See the main text for the Figure of the geometry of the employed slab. The slab structure is also provided in XSF format in Supplementary Table 3.

Supplementary Table 3: Employed slab geometry of TbMn<sub>6</sub>Sn<sub>6</sub> in XSF format (Angstrom units).

| CRYSTAL      |               |               |                |
|--------------|---------------|---------------|----------------|
| PRIMVEC      |               |               |                |
| 4.7891204829 | -2.7650000000 | 0.0000000000  |                |
| 0.0000000000 | 5.5300000000  | 0.0000000000  |                |
| 0.0000000000 | 0.0000000000  | 27.0690000000 |                |
| PRIMCOORD    |               |               |                |
| 23 1         |               |               |                |
| 65           | 0.0000000000  | 0.0000000000  | 13.5345000000  |
| 25           | 2.3945602415  | -1.3825000000 | -6.7446925000  |
| 25           | 2.3945602415  | -4.1475000000 | -6.7446925000  |
| 25           | 0.0000000000  | -2.7650000000 | -6.7446925000  |
| 25           | 2.3945602415  | -1.3825000000 | -11.3013075000 |
| 25           | 2.3945602415  | 1.3825000000  | -11.3013075000 |
| 25           | -0.0000000000 | -2.7650000000 | -11.3013075000 |
| 25           | 2.3945602415  | -1.3825000000 | 11.3013075000  |
| 25           | 2.3945602415  | -4.1475000000 | 11.3013075000  |
| 25           | 0.0000000000  | -2.7650000000 | 11.3013075000  |
| 25           | 2.3945602415  | -1.3825000000 | 6.7446925000   |
| 25           | 2.3945602415  | 1.3825000000  | 6.7446925000   |
| 25           | -0.0000000000 | -2.7650000000 | 6.7446925000   |
| 50           | 0.0000000000  | 0.0000000000  | 10.4883352000  |
| 50           | 0.0000000000  | 0.0000000000  | -7.5576648000  |
| 50           | 0.0000000000  | 0.0000000000  | 7.5576648000   |
| 50           | 0.0000000000  | 0.0000000000  | -10.4883352000 |
| 50           | 1.5963734943  | -2.7650000000 | 13.5345000000  |
| 50           | -1.5963734943 | 2.7650000000  | 13.5345000000  |
| 50           | 1.5963734943  | -2.7650000000 | 9.0230000000   |
| 50           | 1.5963734943  | -2.7650000000 | -9.0230000000  |
| 50           | -1.5963734943 | 2.7650000000  | 9.0230000000   |
| 50           | -1.5963734943 | 2.7650000000  | -9.0230000000  |

\* annaberdiyea@ornl.gov

† subhasish.mandal@mail.wvu.edu

‡ ganeshp@ornl.gov

## SUPPLEMENTARY NOTE 2. PSEUDOPOTENTIALS

### A. Optimization Methods

The objective function  $\mathcal{O}^2$  consists of energy gaps  $\Delta E_{\text{ECP}}^{(s)}$  calculated using CCSD(T) and single-particle orbital eigenvalues  $\epsilon_{\text{ECP}}^{(i)}$  to be matched with the relativistic AE counterparts:

$$\mathcal{O}^2 = \sum_{s \in S} w_s (\Delta E_{\text{AE}}^{(s)} - \Delta E_{\text{ECP}}^{(s)})^2 + \sum_{i \in L} w_i (\epsilon_{\text{AE}}^{(i)} - \epsilon_{\text{ECP}}^{(i)})^2 \quad (1)$$

where  $S$  is the number of considered energy gaps, and  $L$  is the highest occupied angular momentum channel.

Throughout the main text, the ECP errors are assessed via the mean absolute deviation (MAD) from a large set of AE atomic gaps, which include states such as electron affinity, first, second, and third ionization potentials, as well as neutral excitations:

$$\text{MAD} = \frac{1}{N} \sum_i^N |\Delta E_i^{\text{ECP}} - \Delta E_i^{\text{AE}}|. \quad (2)$$

Low-lying gaps such as electron affinity, first ionization potential, and some neutral excitations are also considered:

$$\text{LMAD} = \frac{1}{n} \sum_i^n |\Delta E_i^{\text{ECP}} - \Delta E_i^{\text{AE}}| \quad (3)$$

where  $n < N$ . Finally, a weighted MAD (WMAD) is also shown to capture the biases from all states with an appropriate weight:

$$\text{WMAD} = \frac{1}{N} \sum_i^N \frac{100\%}{\sqrt{|\Delta E_i^{\text{AE}}|}} |\Delta E_i^{\text{ECP}} - \Delta E_i^{\text{AE}}|. \quad (4)$$

### B. Sn ccECP

#### 1. Sn: Transferability Tests

Supplementary Figure 1 shows the Sn atomic spectrum errors for the developed ccECP and various other core approximations with respect to scalar-relativistic AE CCSD(T) data. The plot illustrates the mean absolute deviation (MAD) of a large set of energy gaps, the MAD of low-lying states (LMAD), and a weighted MAD (WMAD), which weights the gaps inverse-proportionally. Previously tabulated ECPs - LANL2 [2], MDFSTU [3], MWBSTU [4], SDFSTU [5], BFD [6], TN-DF [7, 8], CRENBS [9], SBKJJC [10], and their errors are also shown for comparison with ccECP. Here UC stands for uncorrelated core, an AE calculation with the core excitations frozen.

In Supplementary Figure 2, transferability tests are shown using SnH and SnO molecules. Overall, the developed ccECP displays very little error, both in molecular binding and atomic gaps.

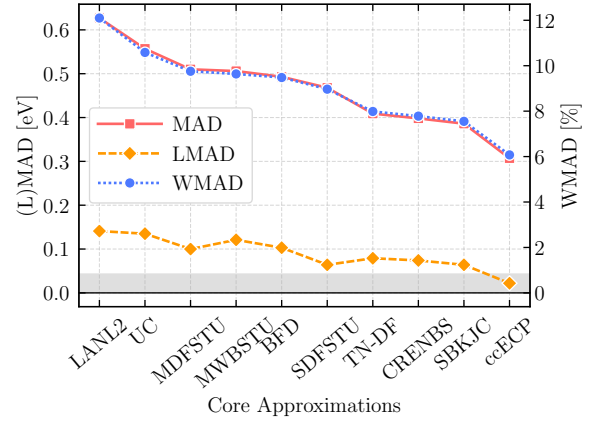

Supplementary Figure 1: Sn atom scalar relativistic AE gap (W/L)MADs for various core approximations. The shaded region represents the chemical accuracy, 1 kcal/mol ( $\approx 0.043$  eV). UCCSD(T) method with uncontracted aug-cc-pVQZ basis set was used.

#### 2. Sn: Atomic Spectrum Errors

Supplementary Table 4 shows the Sn atomic spectrum errors of various core approximations. This data is summarized in Supplementary Figure 1.

In Supplementary Table 5, the full-relativistic ECP errors are shown for ccECP and MDFSTU. These calculations include explicit spin-orbit interactions.

#### 3. Sn: Initial Guess and Optimization

The exponents of Sn ccECP were adopted from SDFSTU and kept frozen during optimizations. A regularizing local channel was added to SDFSTU, and optimizations started from this ECP. Note that SDFSTU was optimized to match the energies of various single-particle states  $n\ell$  with varying numbers of  $n$  and  $\ell$ .

ccECP optimization included orbital eigenvalues and atomic gaps shown in Supplementary Table 4. The UCCSD(T) atomic spectrum overfitting showed underbinding tendency, while eigenvalue overfitting showed overbinding tendency. A good balance between spectrum and eigenvalues was found. The total energy was given a very small weight.

#### 4. Sn: ccECP Parameters

Listing 1 provides the final form of Sn ccECP as AREP and SO terms.

#### 5. Sn: Kinetic Energy Cutoff

Supplementary Table 6 shows the Sn ccECP energy convergence with respect to plane wave cutoff  $E_C$ . Note that  $E_C = 100$  Ry is enough for converged calculations.

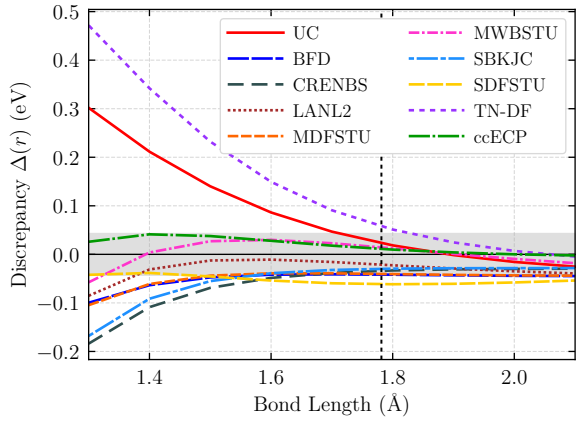

(a) SnH binding curve discrepancies

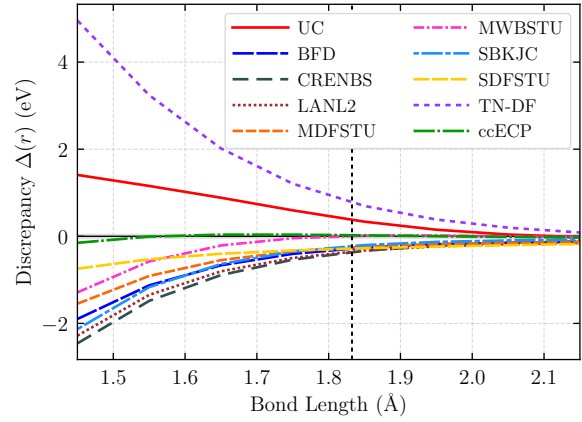

(b) SnO binding curve discrepancies

Supplementary Figure 2: Binding energy discrepancies for (a) SnH and (b) SnO molecules relative to scalar relativistic (DKH) AE UCCSD(T). The shaded region indicates the band of chemical accuracy. The dashed vertical line represents the equilibrium geometry.

Supplementary Table 4: Sn atom scalar relativistic (DKH) AE gaps and relative errors for various core approximations. The core is taken as core=[Kr]4d<sup>10</sup> (46 core, 4 valence electrons). UCCSD(T) method with uncontracted aug-cc-pwCVQZ basis set was used. MAD stands for mean absolute deviation, LMAD is MAD for low-lying states (EA, IP1, IP2), and WMAD is a weighted MAD where the weights are 100%/√|Δ<sup>AE</sup>|. “Q.” represents the charge of the state. All values are in eV.

| State                                 | Q. | AE     | LANL2  | UC     | MDFSTU | MWBSTU | BFD    | SDFSTU | TN-DF  | CRENBS | SBKJC  | ccECP  |
|---------------------------------------|----|--------|--------|--------|--------|--------|--------|--------|--------|--------|--------|--------|
| [core]5s <sup>2</sup> 5p <sup>2</sup> | 0  | 0.000  |        |        |        |        |        |        |        |        |        |        |
| [core]5s <sup>2</sup> 5p <sup>3</sup> | -1 | -1.406 | 0.007  | -0.005 | -0.020 | -0.013 | -0.028 | -0.023 | -0.018 | -0.015 | -0.021 | -0.021 |
| [core]5s <sup>2</sup> 5p <sup>1</sup> | +1 | 7.317  | -0.106 | -0.093 | -0.058 | -0.076 | -0.053 | -0.031 | -0.044 | -0.046 | -0.035 | -0.004 |
| [core]5s <sup>2</sup> 6s <sup>1</sup> | +1 | 13.998 | -0.236 | -0.196 | -0.089 | -0.111 | -0.087 | -0.036 | -0.114 | -0.098 | -0.070 | 0.031  |
| [core]5s <sup>2</sup> 5d <sup>1</sup> | +1 | 14.577 | -1.034 | -0.838 | -0.882 | -0.810 | -0.844 | -0.910 | -0.771 | -0.780 | -0.779 | -0.762 |
| [core]5s <sup>2</sup>                 | +2 | 21.569 | -0.311 | -0.307 | -0.223 | -0.273 | -0.227 | -0.137 | -0.173 | -0.162 | -0.136 | -0.042 |
| [core]5s <sup>1</sup> 5d <sup>1</sup> | +2 | 39.156 | -1.291 | -1.122 | -1.092 | -1.048 | -0.991 | -1.056 | -0.776 | -0.741 | -0.743 | -0.491 |
| [core]5s <sup>1</sup>                 | +3 | 52.080 | -1.407 | -1.334 | -1.210 | -1.208 | -1.220 | -1.085 | -0.964 | -0.945 | -0.915 | -0.798 |
| MAD                                   |    |        | 0.627  | 0.557  | 0.510  | 0.506  | 0.493  | 0.468  | 0.409  | 0.398  | 0.386  | 0.307  |
| LMAD                                  |    |        | 0.141  | 0.135  | 0.100  | 0.121  | 0.103  | 0.064  | 0.079  | 0.074  | 0.064  | 0.022  |
| WMAD[%]                               |    |        | 12.099 | 10.584 | 9.756  | 9.638  | 9.480  | 8.967  | 7.986  | 7.781  | 7.551  | 6.074  |

## 6. Sn: correlation consistent basis set optimization

## C. Tb ccECP

### 1. Tb: Orbital Eigenvalues

AE and ccECP single-particle eigenvalues for low-lying [Xe]4f<sup>9</sup>6s<sup>2</sup> and [Xe]4f<sup>8</sup>5d<sup>1</sup>6s<sup>2</sup> states are listed in Supplementary Tables 7 and 8 respectively. In both cases, the eigenvalues of 4s, 4p, and 4d orbitals are significantly lower than the valence eigenvalues, indicating the validity of the chosen core↔valence partitioning. Also, note that the eigenvalue of 4f seems to be too small to be considered a core state.

### 2. Tb: Atomic Spectrum Errors

Supplementary Table 9 shows the scalar-relativistic Tb atomic spectrum errors for various core approximations. Note that ccECP is accurate up to  $Q = +3$ . As the nominal charge of Tb in the solid is  $Q = +3$ , this indicates that the

Gaussian-type, correlation-consistent basis sets suitable for molecular calculations using quantum chemistry packages were optimized using HF and CCSD(T) methods. The *s* and *p* contraction exponents and coefficients were obtained from HF, while the correlation-consistent terms were optimized by CCSD(T) using an even-tempered scheme. For details of this optimization methodology, see Ref. [11]. (aug)-cc-pVnZ basis sets and ECPs given in MOLPRO, NWCHEM, GAMESS, GAUSSIAN, and DIRAC code formats as well as UPF files for QUANTUM ESPRESSO and XML files for QMCPACK can be found in Ref. [12].

Supplementary Table 5: Sn atomic excitation errors for ccECP versus MDFSTU in SOREP forms. The errors are shown for full-relativistic X2C AE gaps using COSCI. All values are in eV.

| Configuration | Term        | AE     | ccECP   | MDFSTU  |
|---------------|-------------|--------|---------|---------|
| $5s^2 5p^2$   | $^3P_0$     | 0.0000 | 0.0000  | 0.0000  |
|               | $^3P_1$     | 0.1862 | 0.0065  | 0.0187  |
|               | $^3P_2$     | 0.4236 | 0.0083  | 0.0324  |
|               | $^1D_2$     | 1.3200 | -0.0229 | 0.0114  |
|               | $^1S_0$     | 2.7526 | -0.0758 | -0.0269 |
| $5s^2 5p^3$   | $^4S_{3/2}$ | 0.0000 | 0.0000  | 0.0000  |
|               | $^2D_{3/2}$ | 1.1016 | -0.0348 | -0.0278 |
|               | $^2D_{5/2}$ | 1.1654 | -0.0314 | -0.0192 |
|               | $^2P_{1/2}$ | 1.9002 | -0.0520 | -0.0343 |
|               | $^2P_{3/2}$ | 2.0274 | -0.0473 | -0.0192 |
| $5s^2 5p^1$   | $^2P_{1/2}$ | 0.0000 | 0.0000  | 0.0000  |
|               | $^2P_{3/2}$ | 0.5218 | 0.0062  | 0.0378  |
| $5s^2 5d^1$   | $^2D_{3/2}$ | 0.0000 | 0.0000  | 0.0000  |
|               | $^2D_{5/2}$ | 0.0234 | 0.0000  | 0.0037  |
| MAD           |             |        | 0.0285  | 0.0232  |

Listing 1: Sn ccECP parameters in Molpro ECP format.

```

ECP, Sn, 46, 3, 2
4 !ul
1, 2.000000, 4.000000
3, 2.000000, 8.000000
2, 2.000000, -12.706546
2, 1.000000, -0.237233
2 !s
2, 2.000000, 48.172258
2, 1.000000, -4.559077
2 !p
2, 2.000000, 48.856272
2, 1.000000, -1.913865
2 !d
2, 0.666000, 6.850466
2, 0.333000, -0.247154
2 !p-so
2, 2.716017, -2.371998
2, 1.359517, 2.093748
2 !d-so
2, 0.300000, -0.857741
2, 0.520563, 3.223343

```

Supplementary Table 6: QUANTUM ESPRESSO SCF kinetic energy cutoff convergence for Sn ccECP.  $[10 \times 10 \times 10]$  Angstrom cell and PBE functional was used. 100 Ry is enough to achieve 1 meV/e convergence.

| $E_C$ [Ry] | Total Energy [Ry] |
|------------|-------------------|
| 50         | -6.74263240       |
| 100        | -6.74298953       |
| 150        | -6.74300760       |
| 200        | -6.74301096       |

Supplementary Table 7: Tb scalar relativistic (DKH) AE and ccECP eigenvalues [Ha] of  $[\text{Xe}]4f^9 6s^2$  state. RHF method in  $D_{2h}$  point group with uncontracted aug-cc-pwCVTZ basis set was used. Eigenvalues for  $s$ ,  $p_x$ ,  $d_{yz}$ , and  $f_{xyz}$  are shown.

| Orbital | AE         | ccECP   |
|---------|------------|---------|
| 1s      | -1920.3973 |         |
| 2s      | -322.8168  |         |
| 2p      | -287.0796  |         |
| 3s      | -73.4819   |         |
| 3p      | -62.2062   |         |
| 3d      | -47.2270   |         |
| 4s      | -15.4251   |         |
| 4p      | -11.6218   |         |
| 4d      | -6.1995    |         |
| 5s      | -2.1357    | -2.1438 |
| 5p      | -1.1464    | -1.1581 |
| 4f      | -0.4358    | -0.3897 |
| 6s      | -0.1850    | -0.1848 |

Supplementary Table 8: Tb scalar relativistic (DKH) AE and ccECP eigenvalues [Ha] of  $[\text{Xe}]4f^8 5d^1 6s^2$  state. RHF method in  $D_{2h}$  point group with uncontracted aug-cc-pwCVTZ basis set was used. Eigenvalues for  $s$ ,  $p_x$ ,  $d_{xy}$ , and  $f_{xyz}$  are shown.

| Orbital | AE         | ccECP   |
|---------|------------|---------|
| 1s      | -1920.6455 |         |
| 2s      | -323.0878  |         |
| 2p      | -287.3516  |         |
| 3s      | -73.7872   |         |
| 3p      | -62.5295   |         |
| 3d      | -47.5373   |         |
| 4s      | -15.7199   |         |
| 4p      | -11.9329   |         |
| 4d      | -6.4678    |         |
| 5s      | -2.2948    | -2.2946 |
| 5p      | -1.2872    | -1.2882 |
| 4f      | -0.8547    | -0.8501 |
| 5d      | -0.2468    | -0.2589 |
| 6s      | -0.1998    | -0.1984 |

obtained ccECP should be accurately transferable to the solid.

Supplementary Table 10 shows the full-relativistic Tb  $J$ -splitting errors for ccECP. An excellent agreement is obtained within 0.01 eV of the AE data.

### 3. Tb: Initial Guess and Optimization

The following steps were taken to generate a reasonable initial guess for CCSD(T) atomic spectrum optimizations. The idea is to initially separate the optimization into steps that only depend on one non-local channel part of the ECP. In the following steps, all AE calculations use DKH scalar relativity with an uncontracted aug-cc-pwCVTZ basis set.

1. Calculate AE HF state for the “core-configuration” core= $[\text{Kr}]4d^{10}$ .

Supplementary Table 9: Tb scalar relativistic (DKH) AE gaps and relative errors for various core approximations. The core is taken as [Kr]4d<sup>10</sup> (46 core, 19 valence electrons). UCCSD(T) method with uncontracted aug-cc-pwCVTZ basis set was used. MAD stands for mean absolute deviation, LMAD is MAD for 6 low-lying states, and WMAD is a weighted MAD where the weights are 100%/√|Δ<sup>AE</sup>|. All values are in eV. “Q.”

represents the charge of the state. DFT-PBE is an ECP generated using the OPIUM code with a scalar-relativistic PBE and Troullier-Martins scheme.

| State                                                                | Q. | AE      | DFT-PBE | SBKJC  | ccECP  | UC     |
|----------------------------------------------------------------------|----|---------|---------|--------|--------|--------|
| [Xe]4f <sup>8</sup> 6s <sup>2</sup> 5d <sup>1</sup>                  | 0  | 0.000   |         |        |        |        |
| [Xe]4f <sup>9</sup> 6s <sup>2</sup>                                  | 0  | 0.577   | 2.633   | -1.306 | -0.031 | 0.071  |
| [Xe]4f <sup>8</sup> 6s <sup>1</sup> 5d <sup>2</sup>                  | 0  | 1.337   | -0.239  | -0.232 | -0.050 | -0.045 |
| [Xe]4f <sup>8</sup> 6s <sup>2</sup> 6p <sup>1</sup>                  | 0  | 1.776   | 0.299   | -0.511 | -0.027 | 0.039  |
| [Xe]4f <sup>9</sup> 6s <sup>1</sup>                                  | +1 | 6.420   | 2.766   | -1.324 | -0.052 | 0.059  |
| [Xe]4f <sup>8</sup> 6s <sup>1</sup> 5d <sup>1</sup>                  | +1 | 6.204   | -0.020  | -0.342 | -0.037 | -0.018 |
| [Xe]4f <sup>8</sup> 6s <sup>2</sup>                                  | +1 | 6.352   | 0.372   | -0.532 | -0.029 | 0.045  |
| [Xe]4f <sup>9</sup>                                                  | +2 | 17.961  | 3.084   | -1.252 | -0.033 | 0.029  |
| [Xe]4f <sup>8</sup> 5d <sup>1</sup>                                  | +2 | 18.482  | 0.116   | -0.228 | -0.027 | -0.058 |
| [Xe]4f <sup>8</sup> 6s <sup>1</sup>                                  | +2 | 19.316  | 0.452   | -0.534 | -0.072 | 0.024  |
| [Xe]4f <sup>8</sup>                                                  | +3 | 38.934  | 0.723   | -0.386 | -0.064 | -0.021 |
| [Xe]4f <sup>7</sup> 5d <sup>1</sup>                                  | +3 | 44.715  | -3.116  | 1.281  | 0.753  | -0.110 |
| [Xe]4f <sup>7</sup> 6s <sup>1</sup>                                  | +3 | 48.582  | -2.856  | 0.759  | 0.559  | -0.019 |
| [Xe]4f <sup>7</sup>                                                  | +4 | 77.358  | -2.512  | 1.049  | 0.583  | -0.083 |
| [Kr]4d <sup>10</sup> 5s <sup>2</sup> 5p <sup>3</sup> 4f <sup>7</sup> | +7 | 342.117 | -2.841  | -1.209 | -1.262 | -0.502 |
| MAD                                                                  |    |         | 1.573   | 0.782  | 0.256  | 0.080  |
| LMAD                                                                 |    |         | 1.130   | 0.699  | 0.038  | 0.039  |
| WMAD[%]                                                              |    |         | 53.098  | 29.947 | 3.709  | 2.112  |

2. Calculate AE HF state for an “s-only” state. In this case, we used [core]5s<sup>2</sup>6s<sup>2</sup>. The AE valence energy is obtained by subtracting out the core energy from the 1<sup>st</sup> step. Now optimize the s-part of the ECP by matching the total valence energy and orbital eigenvalues of 5s<sup>2</sup> and 6s<sup>2</sup>. All other ECP channel coefficients are set to zero (including the local).
3. Similar to step 2, now obtain AE valence energy for a “p-only” state. We used [core]5p<sup>6</sup> in this case. Again, match the total valence energy and 5p<sup>6</sup> orbital eigenvalue by optimizing the p-part of the ECP.
4. Do similar steps for the d-part of the ECP. We used [core]5d<sup>5</sup> as the reference here.
5. The final non-local channel used is the f-part. Similar steps are repeated for this part using [core]4f<sup>7</sup> reference state.
6. All the optimized parameters from steps 2-5 are combined into one ECP. Now, we have added a local channel, which has been set to zero so far. Again, the local channel is optimized for the total valence energy and orbital eigenvalues of an AE reference state. The reference state was chosen as the trivalent state of [core]5s<sup>2</sup>5p<sup>6</sup>4f<sup>8</sup>6s<sup>2</sup>5d<sup>1</sup>.

In optimization steps 2-5, two Gaussians were used for each step where both exponents and coefficients are optimized. In step 6 (local channel), two Gaussians and two additional Gaussian terms multiplied with 1/*r* and *r* were used, similar to BFD or ccECP parametrizations.

Supplementary Table 10: Tb experimental (Expt.) and all-electron (AE) atomic *J*-splitting gaps due to spin-orbit coupling. ccECP represents the COSCI method errors for SOREP ccECP when compared to full-relativistic X2C AE data. All values are in eV.

| Configuration                                       | Term                                                                                     | Expt.  | AE     | ccECP   |
|-----------------------------------------------------|------------------------------------------------------------------------------------------|--------|--------|---------|
| [Xe]4f <sup>9</sup> 6s <sup>2</sup>                 | <sup>6</sup> H <sub>15/2</sub> <sup>o</sup>                                              | 0.0000 | 0.0000 | 0.0000  |
|                                                     | <sup>6</sup> H <sub>13/2</sub> <sup>o</sup>                                              | 0.3436 | 0.3588 | -0.0022 |
|                                                     | <sup>6</sup> H <sub>11/2</sub> <sup>o</sup>                                              | 0.5791 | 0.6150 | -0.0079 |
|                                                     | <sup>6</sup> H <sub>9/2</sub> <sup>o</sup>                                               | 0.7656 | 0.8121 | -0.0130 |
| [Xe]4f <sup>8</sup> 5d <sup>1</sup> 6s <sup>2</sup> | <sup>8</sup> G <sub>13/2</sub>                                                           | 0.0000 | 0.0000 | 0.0000  |
|                                                     | <sup>8</sup> G <sub>15/2</sub>                                                           | 0.0219 | 0.0075 | 0.0010  |
|                                                     | <sup>8</sup> G <sub>11/2</sub>                                                           | 0.0278 | 0.0580 | 0.0021  |
|                                                     | <sup>8</sup> G <sub>9/2</sub>                                                            | 0.1346 | 0.1716 | 0.0040  |
|                                                     | <sup>8</sup> G <sub>7/2</sub>                                                            | 0.2646 | 0.2863 | 0.0025  |
|                                                     | <sup>8</sup> G <sub>5/2</sub>                                                            | 0.3582 | 0.3751 | -0.0006 |
|                                                     | <sup>8</sup> G <sub>3/2</sub>                                                            | 0.4241 | 0.4399 | -0.0032 |
|                                                     | <sup>8</sup> G <sub>1/2</sub>                                                            | 0.4628 | 0.4792 | -0.0050 |
| [Xe]4f <sup>9</sup> 6s <sup>1</sup>                 | ( <sup>15</sup> / <sub>2</sub> , <sup>1</sup> / <sub>2</sub> ) <sub>8</sub> <sup>o</sup> | 0.0000 | 0.0000 | 0.0000  |
|                                                     | ( <sup>15</sup> / <sub>2</sub> , <sup>1</sup> / <sub>2</sub> ) <sub>7</sub> <sup>o</sup> | 0.1260 | 0.1656 | -0.0391 |
|                                                     | ( <sup>13</sup> / <sub>2</sub> , <sup>1</sup> / <sub>2</sub> ) <sub>7</sub> <sup>o</sup> | 0.3732 | 0.4019 | -0.0301 |
|                                                     | ( <sup>13</sup> / <sub>2</sub> , <sup>1</sup> / <sub>2</sub> ) <sub>6</sub> <sup>o</sup> | 0.4392 | 0.4783 | -0.0224 |
| [Xe]4f <sup>9</sup>                                 | <sup>6</sup> H <sub>15/2</sub> <sup>o</sup>                                              | 0.0000 | 0.0000 | 0.0000  |
|                                                     | <sup>6</sup> H <sub>13/2</sub> <sup>o</sup>                                              | 0.3477 | 0.3593 | -0.0014 |
|                                                     | <sup>6</sup> H <sub>11/2</sub> <sup>o</sup>                                              | 0.5870 | 0.6160 | -0.0068 |
|                                                     | <sup>6</sup> H <sub>9/2</sub> <sup>o</sup>                                               | 0.7759 | 0.8137 | -0.0115 |
|                                                     | <sup>6</sup> H <sub>7/2</sub> <sup>o</sup>                                               | 0.9202 | 0.9660 | -0.0153 |
|                                                     | <sup>6</sup> H <sub>5/2</sub> <sup>o</sup>                                               | 1.0273 | 1.0792 | -0.0182 |
| [Xe]4f <sup>8</sup> 5d <sup>1</sup>                 | <sup>8</sup> G <sub>13/2</sub>                                                           | 0.0000 | 0.0000 | 0.0000  |
|                                                     | <sup>8</sup> G <sub>11/2</sub>                                                           | 0.0305 | 0.0546 | 0.0027  |
|                                                     | <sup>8</sup> G <sub>15/2</sub>                                                           | 0.0376 | 0.0214 | 0.0018  |
|                                                     | <sup>8</sup> G <sub>9/2</sub>                                                            | 0.1361 | 0.1626 | 0.0045  |
|                                                     | <sup>8</sup> G <sub>7/2</sub>                                                            | 0.2509 | 0.2691 | 0.0025  |
|                                                     | <sup>8</sup> G <sub>5/2</sub>                                                            | 0.3356 | 0.3526 | -0.0008 |
|                                                     | <sup>8</sup> G <sub>3/2</sub>                                                            | 0.3959 | 0.4136 | -0.0035 |
|                                                     | <sup>8</sup> G <sub>1/2</sub>                                                            | 0.4317 | 0.4507 | -0.0053 |
| [Xe]4f <sup>8</sup> 6p <sup>1</sup>                 | ( <sup>6</sup> , <sup>1</sup> / <sub>2</sub> ) <sub>11/2</sub> <sup>o</sup>              | 0.0000 | 0.0000 | 0.0000  |
|                                                     | ( <sup>6</sup> , <sup>1</sup> / <sub>2</sub> ) <sub>13/2</sub> <sup>o</sup>              | 0.0265 | 0.0045 | 0.0021  |
|                                                     | ( <sup>5</sup> , <sup>1</sup> / <sub>2</sub> ) <sub>9/2</sub> <sup>o</sup>               | 0.2222 | 0.2260 | 0.0110  |
|                                                     | ( <sup>5</sup> , <sup>1</sup> / <sub>2</sub> ) <sub>11/2</sub> <sup>o</sup>              | 0.3215 | 0.3192 | -0.0147 |
|                                                     | ( <sup>4</sup> , <sup>1</sup> / <sub>2</sub> ) <sub>7/2</sub> <sup>o</sup>               | 0.3628 | 0.3792 | 0.0101  |
|                                                     | ( <sup>4</sup> , <sup>1</sup> / <sub>2</sub> ) <sub>9/2</sub> <sup>o</sup>               | 0.4827 | 0.4918 | -0.0005 |
| MAD                                                 |                                                                                          |        |        | 0.0082  |

All exponents were constrained from below at 1.5 to prevent the generation of long, un-physical potential tails, and they were also constrained from above at 9.0 to prevent very high kinetic energy cut-offs in plane-wave codes. For *f* and local channels, the exponents were constrained from above at 5.0 since it was observed that these channels are the main factors in deciding the plane-wave cut-offs. The same constraints are also applied in the rest of the optimizations as well. To overcome getting trapped in the parameter space, a few starting parameters were tried until small error residuals were obtained.

This concludes the generation of an initial guess to be optimized in CCSD(T) atomic gap optimizations. The rest of the optimization includes atomic spectrum gaps using

Listing 2: Tb ccECP parameters in Molpro ECP format.

```

ECP,Tb,46,4,3
4 !ul
1, 4.526254, 19.000000
3, 3.879308, 85.998831
2, 4.406058, -85.722649
2, 1.899664, -3.133952
2 !s
2, 8.996757, 161.119164
2, 5.104371, 89.334835
2 !p
2, 7.640657, 88.693021
2, 3.878305, 57.109488
2 !d
2, 7.456305, 55.901690
2, 2.530445, 29.364333
2 !f
2, 4.939345, -23.952530
2, 3.912490, -7.090915
1 !p-so
4, 2.080465, 2.963688
1 !d-so
4, 2.660751, 0.922456
1 !f-so
4, 4.708055, 0.178089

```

CCSD(T), eigenvalues of neutral and charge= +3 trivalent states, and the norm for a chosen neutral state.

#### 4. Tb: ccECP Parameters

Listing 2 provides the final form of Tb ccECP as AREP and SO terms.

#### 5. Tb: Kinetic Energy Cutoff

Supplementary Table 11 shows the Tb ccECP energy convergence with respect to plane wave cutoff  $E_C$ . Note that  $E_C = 600$  Ry is enough for converged calculations.

Supplementary Table 11: QUANTUM ESPRESSO SCF kinetic energy cutoff convergence for Tb ccECP.  $[10 \times 10 \times 10]$  Angstrom cell is used with PBE functional. 600 Ry is enough to achieve 1 meV/e convergence.

| $E_C$ [Ry] | Total Energy [Ry] |
|------------|-------------------|
| 300        | -258.21011528     |
| 400        | -258.82039730     |
| 500        | -258.87654695     |
| 600        | -258.88182883     |
| 700        | -258.88237251     |
| 800        | -258.88243440     |

#### 6. Tb: correlation consistent basis set optimization

For the optimization of Gaussian-type, correlation-consistent basis sets for molecular calculations using quantum chemistry methods, we follow a methodology similar to what is described in the Supplemental of Ref. [13]. Briefly, the contraction exponents were first optimized via HF for the trivalent state  $[\text{Xe}]4f^85d^16s^2$  of Tb. Next, we use a CI calculation of this trivalent state to obtain the atomic natural orbitals and use these as contractions for  $s$ ,  $p$ ,  $d$ , and  $f$  channels. By freezing excitations from the  $5s$  and  $5p$  orbitals, we optimize valence-only correlation-consistent and polarization terms using CI to form cc-pVnZ basis sets. Then, an extra “core” term is added to each channel by optimizing the full space in CI to form the cc-pCVnZ basis sets. For the final form of these basis sets, see Ref. [12] where they can be found in MOLPRO, NWCHEM, GAMESS, GAUSSIAN, and DIRAC code formats as well as UPF format for QUANTUM ESPRESSO and XML format for QMCPACK.

### SUPPLEMENTARY NOTE 3. DFT+*U* METHODS AND DATA

Supplementary Tables 12, 13, 14 provide the data for convergence of Gaussian spreading, kinetic energy cutoff, and  $k$ -mesh DFT parameters, respectively. Fully-converged bulk calculation parameters used in the study are 0.001 Ry Gaussian spreading, 600 Ry kinetic energy cutoff, and  $[8 \times 8 \times 8]$   $k$ -mesh in the bulk primitive cell. Slab calculations used  $[8 \times 8 \times 1]$   $k$ -mesh in the SCF calculations, which were observed to be converged with respect to  $k$ -mesh. Hybrid DFA calculations employed a smaller  $[4 \times 4 \times 4]$   $k$ -mesh due to the high cost of hybrids in bulk systems.

Supplementary Table 12: Convergence of QUANTUM ESPRESSO Gaussian spreading (Ry) for Brillouin-zone integration in bulk TbMn<sub>6</sub>Sn<sub>6</sub>.  $k$ -mesh =  $[2 \times 2 \times 1]$ . PBE functional. 600 Ry kinetic energy cutoff. Unconstrained total spin magnetization. 0.001 Ry Gaussian spreading was chosen to be used throughout the study.

| Spreading [Ry] | Total Energy [Ry] | $M^s$ [ $\mu_B$ ] |
|----------------|-------------------|-------------------|
| 0.0080         | -1549.08702247    | 10.39             |
| 0.0040         | -1549.07374172    | 8.97              |
| 0.0020         | -1549.07044686    | 9.02              |
| 0.0010         | -1549.06951107    | 9.08              |
| 0.0005         | -1549.06922402    | 9.02              |
| 0.0001         | -1549.06902797    | 9.00              |

Supplementary Table 13: Convergence of QUANTUM ESPRESSO SCF kinetic energy cutoff in bulk TbMn<sub>6</sub>Sn<sub>6</sub>.  $k$ -mesh =  $[2 \times 2 \times 1]$ . PBE functional. Unconstrained total spin magnetization. 600 Ry was chosen to be used throughout the study.

| $E_C$ [Ry] | Total Energy [Ry] | $M^s$ [ $\mu_B$ ] |
|------------|-------------------|-------------------|
| 400        | -1549.00725031    | 9.09              |
| 450        | -1549.04997024    | 9.09              |
| 500        | -1549.06357348    | 9.09              |
| 550        | -1549.06803239    | 9.08              |
| 600        | -1549.06951102    | 9.08              |
| 650        | -1549.07005881    | 9.08              |

To facilitate the SCF convergence in the large  $k$ -mesh calculations, we first converged the calculations in a coarse  $k$ -mesh of  $[2 \times 2 \times 1]$ . We then carried out non-self-consistent calculations (nscf) for a desired dense  $k$ -mesh using the charge densities from the previous coarse  $k$ -mesh. The resulting orbitals from the nscf and the previously obtained charge density were given as an initial guess to the dense  $k$ -mesh SCF, which showed very robust convergence behavior.

Supplementary Table 15 shows the effect of applying Hubbard  $U$  on Mn-3*d*, Tb-4*f*, Tb-5*d*, and Sn-5*p* orbitals. Note that there are significant changes in magnetic moments and cell magnetizations when  $U$  is applied on Mn-3*d* orbitals. However, the corresponding changes are much smaller when  $U$  is applied to other subspaces. This is further explored by plotting the band structure of TbMn<sub>6</sub>Sn<sub>6</sub> when a  $+U$  is applied on Tb 4*f* orbitals in addition to the

Mn 3*d* orbitals. Supplementary Figure 3 shows this band structure using LDA+ $U_{\text{Mn}}^{3d}$  (−0.5 eV)+ $U_{\text{Tb}}^{4f}$  (1.0 eV) DFA. We observe that this band structure is indistinguishable to the human eye from the band structure given in the main text, where the  $+U$  is not applied on Tb 4*f* orbitals. This indicates that Tb 4*f* orbitals are already sufficiently localized, and the application of  $+U_{\text{Tb}}^{4f}$  is not crucial for this study, where we focus on small energy scales around  $E_F$ .

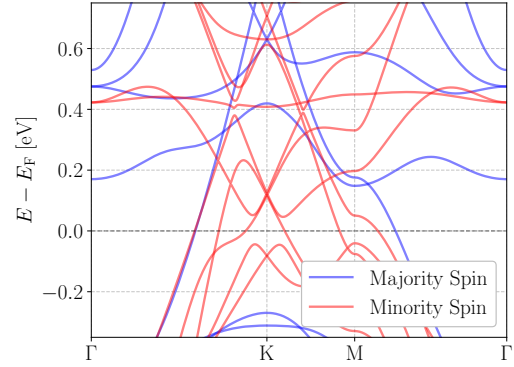

Supplementary Figure 3: Bulk band structure of TbMn<sub>6</sub>Sn<sub>6</sub> when an additional  $+U$  is applied on Tb 4*f* orbitals besides the Mn 3*d* orbitals. Here the DFA is LDA+ $U_{\text{Mn}}^{3d}$  (−0.5 eV)+ $U_{\text{Tb}}^{4f}$  (1.0 eV). This band structure is indistinguishable from the bands in the main text, where  $+U_{\text{Tb}}^{4f} = 0$ .

Supplementary Figure 4 shows the extraction of the Dirac velocity ( $v_D$ ). The Dirac velocity is obtained using a fit to the Dirac dispersion in the presence of a Chern gap due to SOC [14] near  $k = K$  point:

$$E_k = E_{\text{DC}} \pm \sqrt{(\Delta/2)^2 + (\hbar k v_D)^2} \quad (5)$$

The fit range was chosen as  $[-0.05, 0.05] 2\pi/a$  where  $a = 10.45018551$  Bohr is a lattice parameter. This procedure gives  $v_D = 2.25 \times 10^5$  m/s. We have also calculated the  $v_D$  using the linear Dirac dispersion:

$$E_k = E_{\text{DC}} \pm \hbar k v_D \quad (6)$$

by numerical differentiation near  $k = K$  which resulted in a similar  $v_D$  as above.

In Supplementary Figure 5, the Fermi surfaces of bulk TbMn<sub>6</sub>Sn<sub>6</sub> using scalar-relativistic LDA+ $U_{\text{Mn}}^{3d}$  (−0.5 eV) is shown. To obtain the Fermi surface, an SCF calculation with a  $[8 \times 8 \times 8]$   $k$ -mesh and a non-SCF calculation with a larger  $[20 \times 20 \times 20]$   $k$ -mesh was used. The Fermi surfaces are shown for the majority and minority spin channels.

Supplementary Figure 6, and Supplementary Figure 7 demonstrate how the atomic moments and charges, respectively, change as different  $U_{\text{Mn}}^{3d}$  values are applied on LDA using averaged SOC effects (AREP). Supplementary Figure 8 shows the Mn atomic moment and cell magnetization as  $J$  is included.

Supplementary Figures 9, 10, and 10 demonstrate the bulk, subsurface, and surface band structures obtained via projections into the atomic Mn-*d* orbitals. Specifically, these are plotted using the  $k$ -resolved, partial density of

Supplementary Table 14: Convergence of QUANTUM ESPRESSO SCF  $k$ -mesh in bulk TbMn<sub>6</sub>Sn<sub>6</sub>. PBE functional. Unconstrained total spin magnetization ( $M^s$  [ $\mu_B$ ]). 600 Ry kinetic energy cutoff. Approximate spin magnetic moments  $m^s$  [ $\mu_B$ ] (integrated on an atomic sphere of a certain radius) are shown for each species.  $m_{\text{Sn}}^s$  values are averaged over 3 slightly different values (of range  $\approx 0.01\mu_B$ ).  $E_F$  is the Fermi level.  $[8 \times 8 \times 8]$   $k$ -mesh was used throughout the study.

| $k$ -mesh                  | Total Energy [Ry] | $m_{\text{Tb}}^s$ | $m_{\text{Mn}}^s$ | $m_{\text{Sn}}^s$ | $M^s$ | $ M^s $ | $E_F$ [eV] |
|----------------------------|-------------------|-------------------|-------------------|-------------------|-------|---------|------------|
| $[2 \times 2 \times 2]$    | -1549.05326051    | -6.2141           | 2.7677            | -0.1021           | 9.32  | 24.70   | 11.8286    |
| $[4 \times 4 \times 4]$    | -1549.05680281    | -6.2488           | 2.6583            | -0.1071           | 8.44  | 24.20   | 11.7608    |
| $[6 \times 6 \times 6]$    | -1549.05705150    | -6.2519           | 2.6522            | -0.1115           | 8.33  | 24.22   | 11.7640    |
| $[8 \times 8 \times 8]$    | -1549.05700751    | -6.2518           | 2.6345            | -0.1141           | 8.17  | 24.13   | 11.7561    |
| $[10 \times 10 \times 10]$ | -1549.05679211    | -6.2507           | 2.6346            | -0.1134           | 8.19  | 24.12   | 11.7544    |
| $[12 \times 12 \times 12]$ | -1549.05661464    | -6.2509           | 2.6335            | -0.1136           | 8.18  | 24.12   | 11.7545    |

Supplementary Table 15: The effect of applying Hubbard  $+U$  on Tb  $4f$ ,  $5d$ , and Sn  $5p$  subspaces. LDA+ $U$ [eV] DFA with unconstrained total spin magnetization ( $M^s$  [ $\mu_B$ ]) is used. 600 Ry kinetic energy cutoff. Approximate spin magnetic moments  $m^s$  [ $\mu_B$ ] (integrated on an atomic sphere of a certain radius) are shown for each species.  $m_{\text{Sn}}^s$  values are averaged over 3 slightly different values.  $E_F$  is the Fermi level.  $[8 \times 8 \times 8]$   $k$ -mesh was used in this table.

| $U_{\text{Mn}}^{3d}$ | $U_{\text{Tb}}^{4f}$ | $U_{\text{Tb}}^{5d}$ | $U_{\text{Sn}}^{5p}$ | $m_{\text{Tb}}^s$ | $m_{\text{Mn}}^s$ | $m_{\text{Sn}}^s$ | $M^s$ | $ M^s $ |
|----------------------|----------------------|----------------------|----------------------|-------------------|-------------------|-------------------|-------|---------|
| 0.5                  | 0.0                  | 0.0                  | 0.0                  | -6.2550           | 2.9040            | -0.1002           | 10.20 | 25.54   |
| 0.0                  | 0.0                  | 0.0                  | 0.0                  | -6.2601           | 2.3954            | -0.0924           | 7.09  | 22.33   |
| -0.5                 | 0.0                  | 0.0                  | 0.0                  | -6.2282           | 2.2498            | -0.0761           | 6.51  | 21.19   |
| -0.5                 | 1.0                  | 0.0                  | 0.0                  | -6.2359           | 2.2515            | -0.0761           | 6.51  | 21.21   |
| -0.5                 | -1.0                 | 0.0                  | 0.0                  | -6.2139           | 2.2474            | -0.0759           | 6.52  | 21.16   |
| -0.5                 | 0.0                  | 1.0                  | 0.0                  | -6.2221           | 2.2481            | -0.0759           | 6.50  | 21.18   |
| -0.5                 | 0.0                  | -1.0                 | 0.0                  | -6.2312           | 2.2516            | -0.0763           | 6.52  | 21.20   |
| -0.5                 | 0.0                  | 0.0                  | 1.0                  | -6.2285           | 2.2549            | -0.0791           | 6.50  | 21.26   |
| -0.5                 | 0.0                  | 0.0                  | -1.0                 | -6.2277           | 2.2458            | -0.0732           | 6.53  | 21.14   |

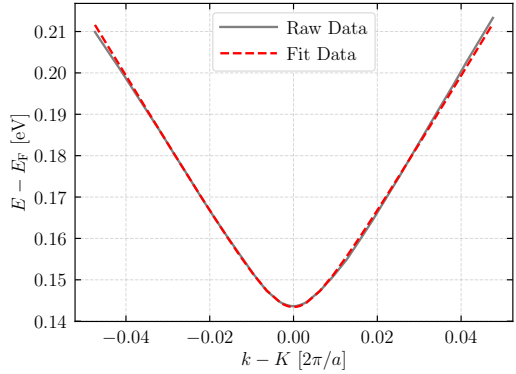

Supplementary Figure 4: Extraction of the Dirac velocity using a fit to the Dirac dispersion in the presence of SOC. The dashed red line is expressed as Equation 5. See the accompanying text for details.

states (pDOS) averaged over different Mn sites:

$$\text{pDOS}^{\langle \text{Mn} \rangle} = \sum_i^N \text{pDOS}^{\text{Mn}}_i(k, E)/N \quad (7)$$

where  $N = 6$  is the number of Mn sites.

Supplementary Figure 12 shows how the band structures change as  $k_z$  is varied for the same path in  $k_x$  and  $k_y$ .

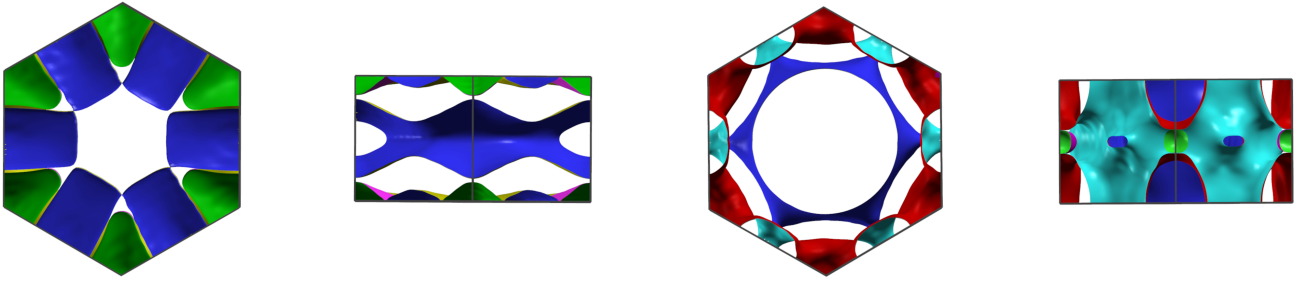

(a) Majority Spin (top view) (b) Majority Spin (side view) (c) Minority Spin (top view) (d) Minority Spin (side view)

Supplementary Figure 5: Fermi surfaces of  $\text{TbMn}_6\text{Sn}_6$  bulk using  $\text{LDA}+U_{\text{Mn}}^{3d}(-0.5 \text{ eV})$ . (a, b) Majority Spin, (c, d) Minority Spin.

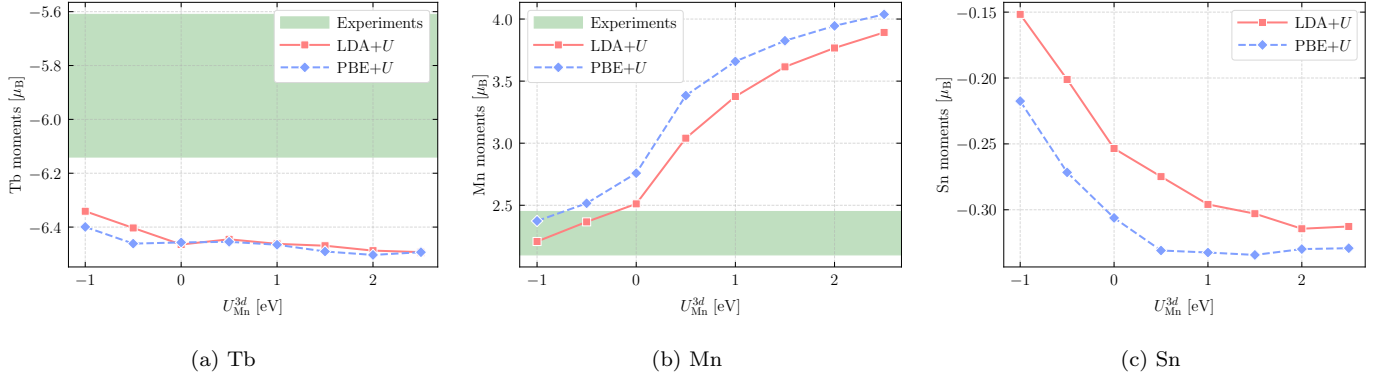

Supplementary Figure 6:  $\text{LDA}+U_{\text{Mn}}^{3d}$  Löwdin atomic moments of (a) Tb, (b) Mn, and (c) Sn as the  $U_{\text{Mn}}^{3d}$  is varied. Sn values are the averages of three different Sn sites. AREP pseudopotentials are used in these plots.

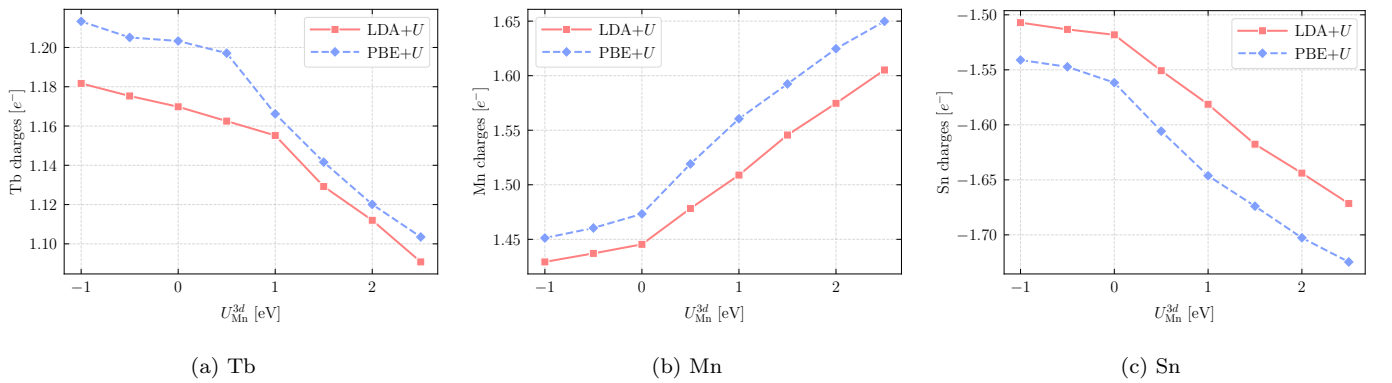

Supplementary Figure 7:  $\text{LDA}+U_{\text{Mn}}^{3d}$  Löwdin atomic effective charges of (a) Tb, (b) Mn, and (c) Sn as the  $U_{\text{Mn}}^{3d}$  is varied. Sn values are the averages of three different Sn sites. AREP pseudopotentials are used in these plots.

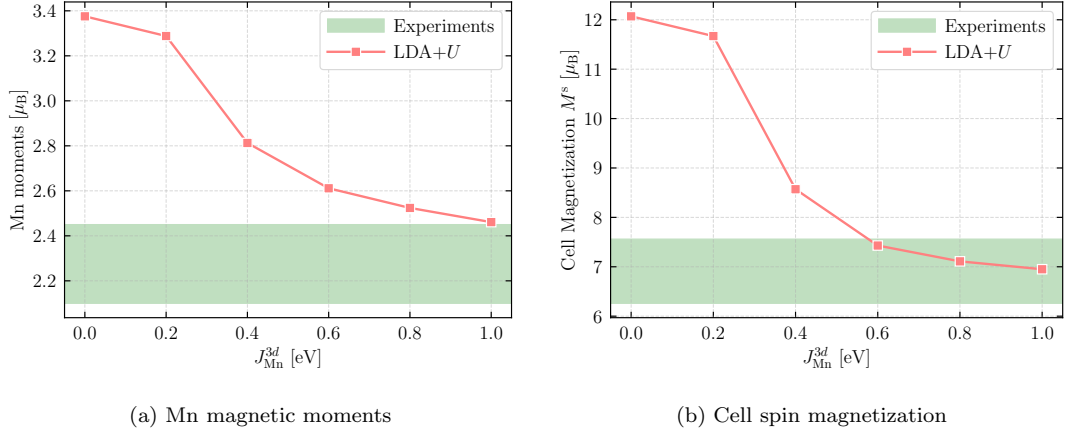

Supplementary Figure 8: Comparison of DFT+ $U + J$  and experimental magnetizations. In these plots,  $U_{\text{Mn}}^d = 1$  eV is fixed, while the  $J_{\text{Mn}}^{3d}$  is varied. (a) Mn atomic magnetic moments, (b) cell spin magnetization per formula unit. The green-shaded regions represent the envelope of various experimental measurements [1, 14–19]. In (b), the experimental cell magnetization was added with the Tb orbital magnetization of  $M_{\text{Tb}}^{\text{orb}} = 2.96 \mu_{\text{B}}$  [20] for a proper comparison,  $M^s = M_{\text{exp}}^{\text{total}} + M_{\text{Tb}}^{\text{orb}}$ .

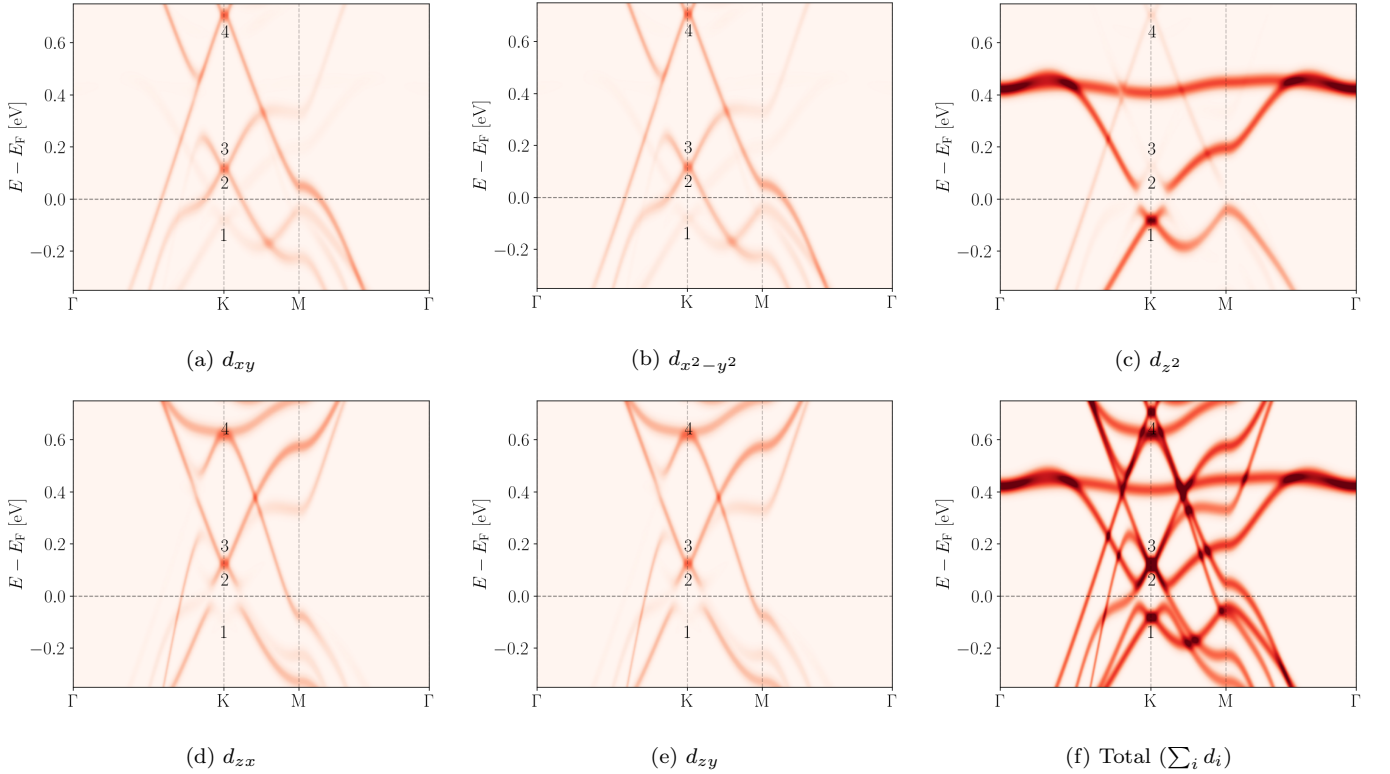

Supplementary Figure 9: Minority spin bulk band structures using projections on the atomic Mn  $d$  orbitals. The plots show the averages over different Mn atoms.

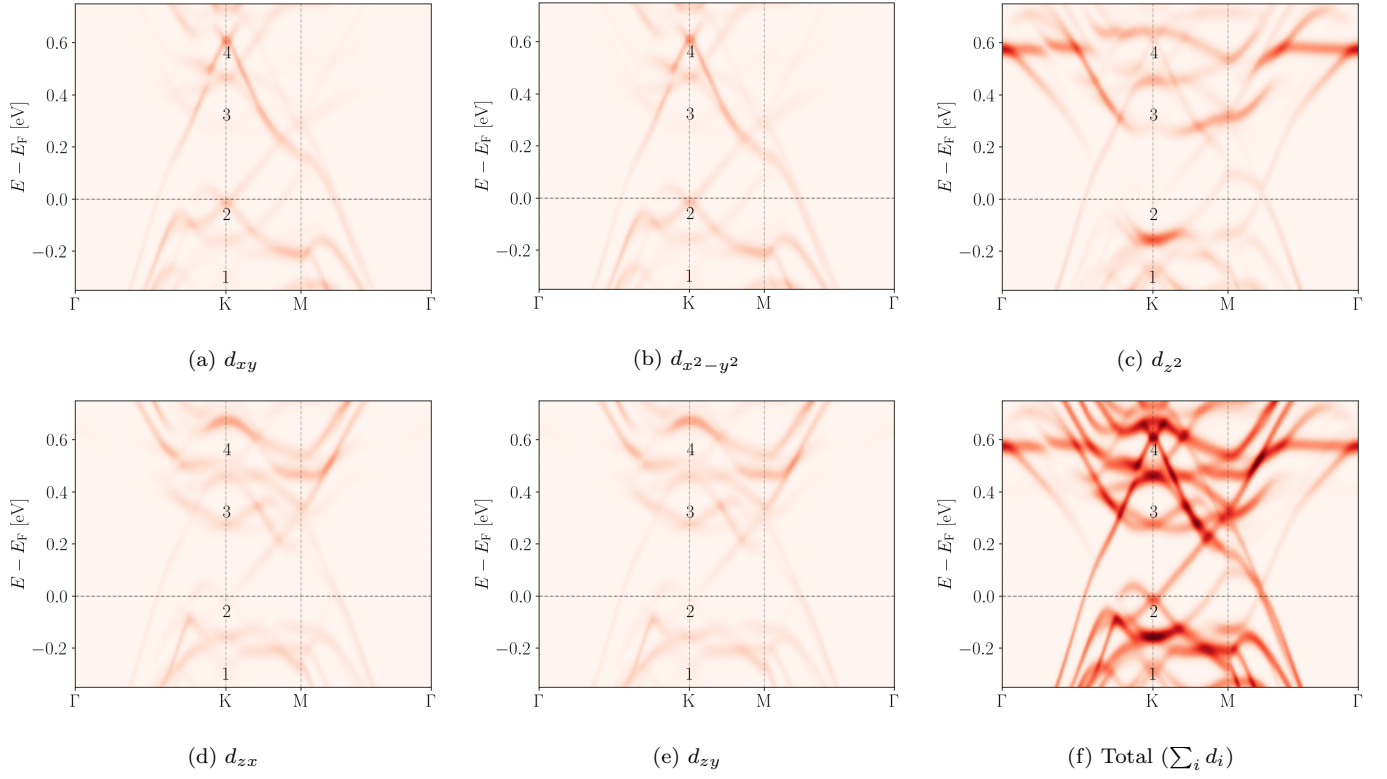

Supplementary Figure 10: Minority spin slab band structures using projections on the *subsurface* atomic Mn  $d$  orbitals. The plots show the averages over different subsurface Mn atoms.

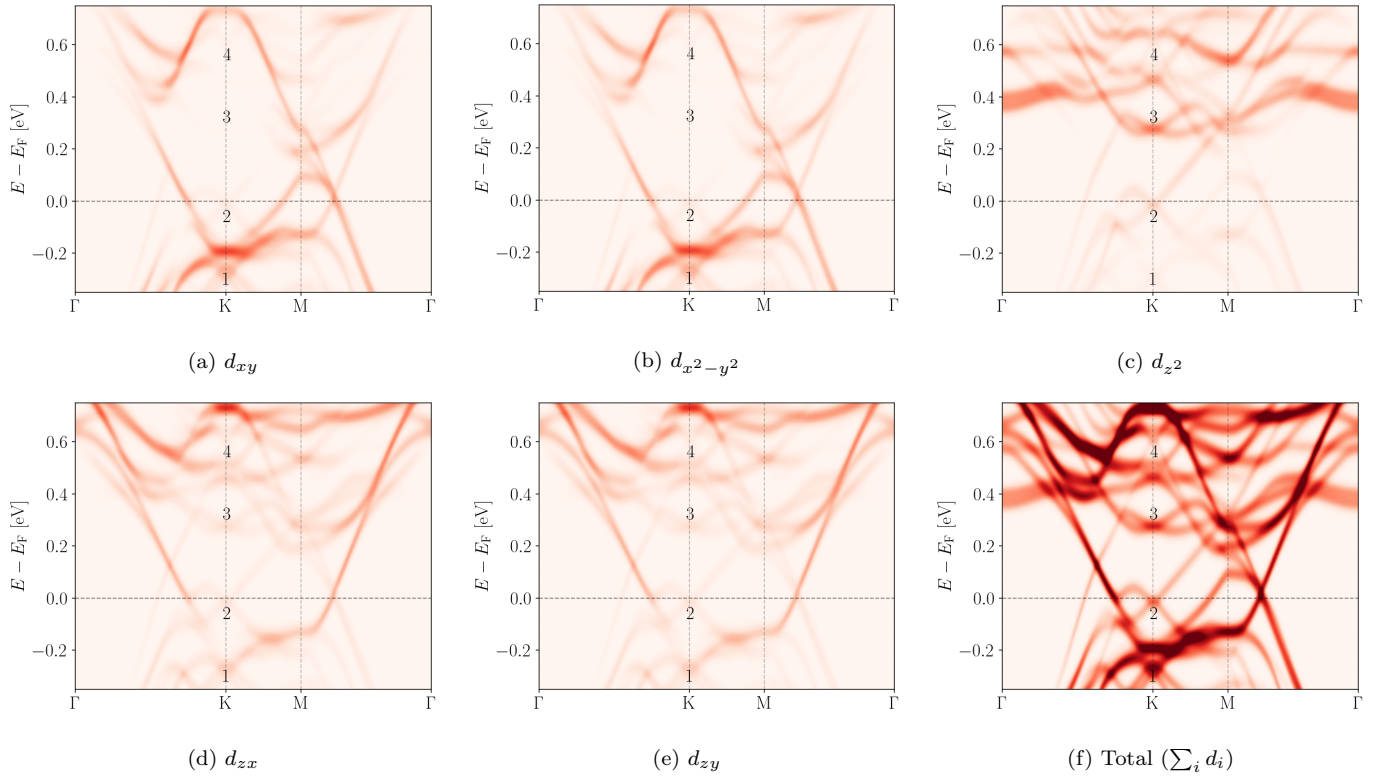

Supplementary Figure 11: Minority spin slab band structures using projections on the *surface* atomic Mn  $d$  orbitals. The plots show the averages over different surface Mn atoms.

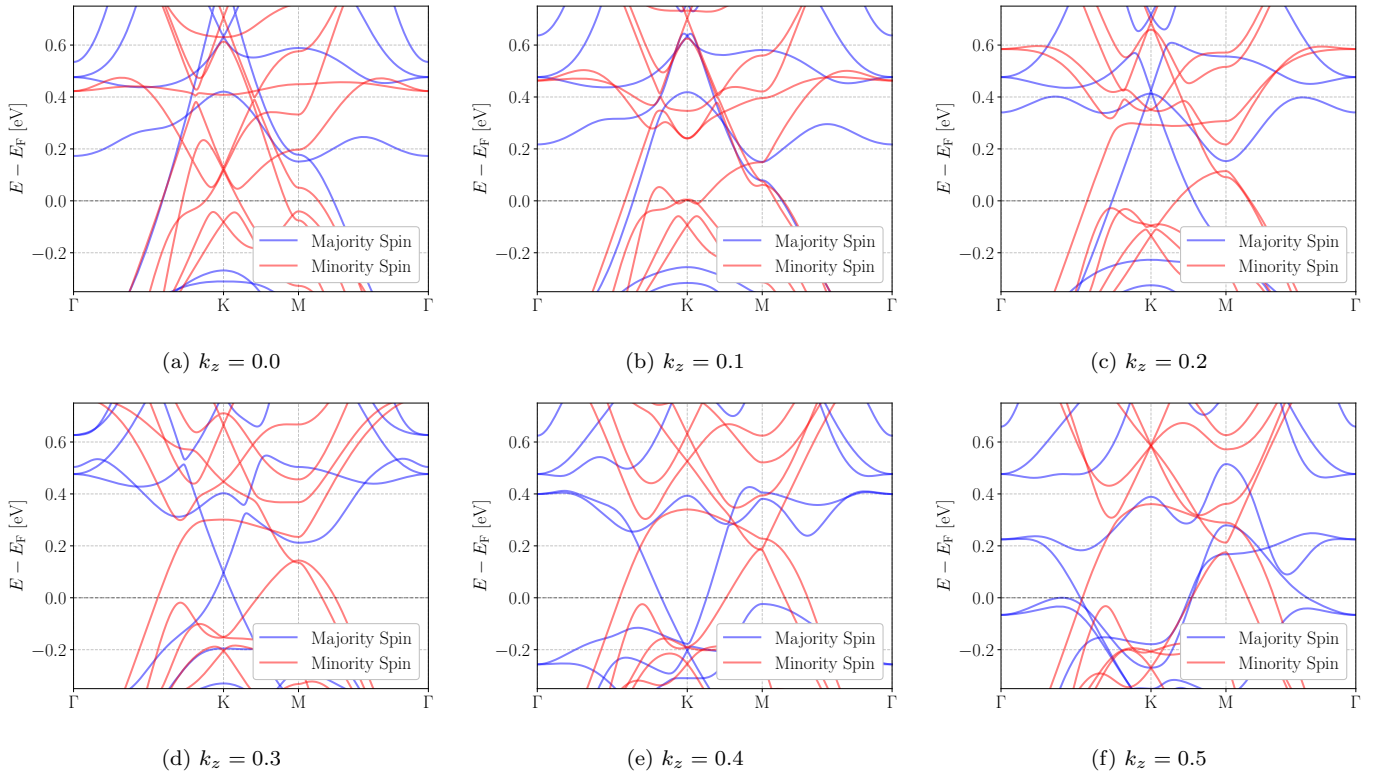

Supplementary Figure 12: Bulk band structures of  $\text{TbMn}_6\text{Sn}_6$  for various  $k_z$  values in reciprocal lattice units. The  $k_z = 0$  labels  $\Gamma$ , K, M are repeated for  $k_z \neq 0$  values for ease of comparison. Note the heavy  $k_z$  dispersion of the bands.

#### SUPPLEMENTARY NOTE 4. QMC METHODS AND DATA

Supplementary Figure 13 shows the DMC timestep extrapolation for  $\text{Tb}^{3+}$  cation. The extrapolated energy is within the error bars of  $\tau = 0.001 \text{ Ha}^{-1}$ ; therefore, this timestep was used for all molecular systems for comparison with the CCSD(T) method. For bulk QMC calculations where we don't compare with CCSD(T), we use a larger  $\tau = 0.02 \text{ Ha}^{-1}$  timestep.

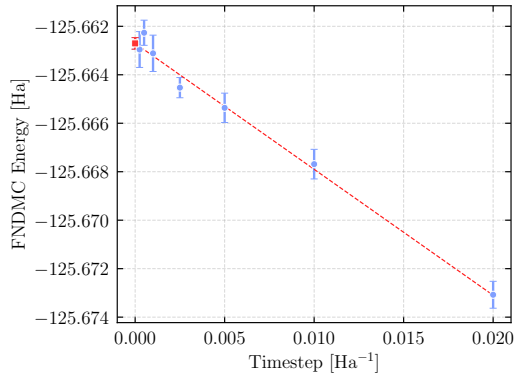

Supplementary Figure 13: DMC timestep extrapolation for  $\text{Tb}^{3+}$  cation. QMC error bars correspond to one standard deviation.

Supplementary Table 16 shows how the total energy converges as the number of integration points for non-local ECP evaluation is increased. We find that a larger number of integration points is required for Tb compared to Mn. For sufficiently dense sampling, we see that the VMC energy agrees with ROHF energy. All DMC calculations use the T-moves algorithm [21] in sampling the non-local part of the ECPs.

Supplementary Table 16: Total energies [Ha] and variances [ $\text{Ha}^2$ ] using VMC with ROHF Slater-determinant trial wave function (no Jastrows). N(quad) is the number of integration points for non-local ECP evaluation in VMC. Exact (ROHF/cc-pVTZ) energy is also shown for comparison. Note that a higher N(quad) is needed for Tb (N(quad)= 26) when compared to Mn (N(quad)= 12).

| N(quad) | Tb(var)  | Tb(en)       | Mn(var)  | Mn(en)       |
|---------|----------|--------------|----------|--------------|
| 12      | 374.4(5) | -126.279(2)  | 12.60(5) | -103.2240(2) |
| 18      | 140.0(2) | -126.280(1)  | 12.60(5) | -103.2240(2) |
| 26      | 17.76(2) | -126.2507(4) | 12.60(5) | -103.2241(2) |
| 32      | 17.80(4) | -126.2504(4) | 12.60(5) | -103.2241(3) |
| 50      | 17.76(3) | -126.2502(4) | 12.60(5) | -103.2241(2) |
| ROHF    |          | -126.25074   |          | -103.22389   |

Orbitals in QMC calculations were represented by a B-spline mesh. The quality of the mesh was tested by comparing it against a hybrid orbital of localized and B-spline representation, see Supplementary Table 18. Note that the employed full B-spline representation results in the same energy as the hybrid representation, showing that the spline mesh is sufficiently dense.

DMC and UCCSD(T) binding energies are shown for  $\text{TbH}_3$  and  $\text{TbO}$  molecules in Supplementary Table 17. In  $\text{TbH}_3$ , the SCF binding energies (HF, PBE0, PBE) show significant variation, but DMC produces the correct  $D_e$  irrespective of the reference trial wave function. An even larger range of SCF predictions can be seen in  $\text{TbO}$ , and DMC values are again in proximity with each other and with overall 0.15 – 0.35 eV (2.0% – 4.5%) underestimation of  $D_e$ . This shows that the  $\text{TbO}$  trial wave function needs to be improved; nevertheless, the agreement is satisfactory, especially when PBE is used to generate the singe-reference trial wavefunction for DMC.

Supplementary Table 17: Binding energies  $D_e$  [eV] of  $\text{TbH}_3$  and  $\text{TbO}$  without the zero-point-energy (ZPE) contributions. HF, PBE0, PBE, and DMC values using these references are shown. UCCSD(T) value is in the CBS limit and can be considered as the near-exact value. DMC and UCCSD(T) energies for O atom were obtained from Ref. [22].

| Method   | $\text{TbH}_3$ | $\text{TbO}$ |
|----------|----------------|--------------|
| HF       | 6.17           | 4.04         |
| PBE0     | 8.52           | 7.26         |
| PBE      | 8.62           | 8.10         |
| DMC/HF   | 8.30(1)        | 7.19(2)      |
| DMC/PBE0 | 8.29(2)        | 7.32(2)      |
| DMC/PBE  | 8.31(1)        | 7.38(2)      |
| UCCSD(T) | 8.34           | 7.53         |

Supplementary Table 19 provides the total energies of  $\text{TbMn}_6\text{Sn}_6$  relevant systems using various methods. Single-reference biases present in QMC calculations were estimated using these total energies.

In Supplementary Figures 14 and 15, we show the VMC energy extrapolations with respect to energy variance for molecular systems considered in this work. All Jastrow factors were optimized using energy minimization. In Supplementary Figure 14, the extrapolations use two data points: Slater determinant and Slater-Jastrow with up to three body terms ( $\text{SJ}_{123}$ ). Here, the extrapolated VMC energy is usually below the DMC/ $\text{SJ}_{123}$  and above the nearly-exact UCCSD(T)/CBS. The notable exception is the Sn atom, where the extrapolated energy is slightly below the exact energy (by about  $10^{-4} \text{ Ha}$ ) since the fixed-node biases are very small. To show that the VMC energy scales linearly in this energy range, we also plot the extrapolations using three data points: Slater,  $\text{SJ}_{12}$ , and  $\text{SJ}_{123}$ . We can see that these points mostly obey the linear regime, and there are no significant changes. In the main text, we have opted to use a two-data point extrapolation, allowing us to achieve better signals in energy comparisons.

Supplementary Table 18: Probe of QMCPACK orbital representation quality in bulk  $\text{TbMn}_6\text{Sn}_6$ . Orbitals can be represented with either full B-spline mesh or a hybrid combination of localized atomic basis set around atomic cores and B-splines. The hybrid representation allows for the use of coarser B-spline mesh. The table below shows whether hybrid representation is used or not for each atomic species. Due to memory constraints, a maximum value of 0.9 could be used for the mesh factor. Maximum spherical harmonics ( $l_{\text{max}}$ ) used for each species are Tb: 6, Mn: 5 with a cutoff radius of 1.5 Bohr.

| Mesh Factor | Tb-hybrid | Mn-hybrid | Sn-hybrid | Total Energy [Ha] | Kinetic Energy [Ha] | Variance [Ha <sup>2</sup> ] |
|-------------|-----------|-----------|-----------|-------------------|---------------------|-----------------------------|
| 0.9         | No        | No        | No        | -1540.013(1)      | 1000.52(2)          | 33.54(8)                    |
| 0.7         | Yes       | Yes       | No        | -1540.015(1)      | 1000.56(3)          | 29.93(2)                    |
| 0.8         | Yes       | Yes       | No        | -1540.016(1)      | 1000.66(3)          | 29.99(9)                    |
| 0.9         | Yes       | Yes       | No        | -1540.012(1)      | 1000.59(3)          | 29.95(5)                    |

Supplementary Table 19: Estimation of combined FN and localization biases in single-reference DMC calculations for  $\text{TbMn}_6\text{Sn}_6$  relevant systems. Total energies [Ha] using various methods are shown. Uncontracted aug-cc-p(wC)VnZ basis sets were used in the extrapolations with  $nZ \in (\text{DZ-QZ})$  for Tb systems and  $nZ \in (\text{TZ-5Z})$  for Sn and Mn atoms.  $0.001 \text{ Ha}^{-1}$  timestep and aug-cc-pVTZ basis sets were used in all DMC calculations. In DMC, T-moves [21] and locality-approximation (LA) [23] algorithms are used for evaluating non-local ECPs. Var/Energy [Ha] is the DMC/ROHF (T-moves) variance to energy ratio.  $\epsilon$  [mHa] represents the DMC/ROHF (T-moves) error compared to UCCSD(T)/CBS,  $\epsilon = (E_{\text{DMC}} - E_{\text{exact}})$ .  $\eta$  is the missing percentage of the correlation energy  $\eta = 100\% \cdot \epsilon / |E_{\text{corr}}|$ . SCF calculations are of spin-restricted type, ROHF or RKS.

| Method           | NL-Eval | Tb <sup>3+</sup> | Tb           | TbH <sub>3</sub> | TbO          | Mn           | Sn         |
|------------------|---------|------------------|--------------|------------------|--------------|--------------|------------|
| ROHF/CBS         |         | -124.9172        | -126.2515    | -127.9783        | -142.0898    | -103.2242    | -3.2736    |
| UCCSD(T)/CBS     |         | -125.7634        | -127.1967    | -129.0033        | -143.3574    | -103.8704    | -3.3438    |
| DMC/HF           | T-moves | -125.6628(3)     | -127.0819(3) | -128.8869(4)     | -143.2157(6) | -103.8130(4) | -3.3422(1) |
| DMC/PBE0         | T-moves | -125.6537(3)     | -127.0723(3) | -128.8769(6)     | -143.2109(5) | -103.8162(3) | -3.3424(1) |
| DMC/PBE          | T-moves | -125.6478(3)     | -127.0651(3) | -128.8705(4)     | -143.2027(5) | -103.8163(3) | -3.3425(1) |
| DMC/HF           | LA      | -125.6829(4)     | -127.1054(4) | -128.9105(7)     | -143.2500(5) | -103.8166(3) | -3.3435(1) |
| DMC/PBE0         | LA      | -125.6740(4)     | -127.0979(4) | -128.9041(5)     | -143.2489(6) | -103.8204(3) | -3.3435(1) |
| DMC/PBE          | LA      | -125.6696(4)     | -127.0914(4) | -128.8979(5)     | -143.2403(6) | -103.8206(4) | -3.3434(1) |
| Var/Energy [Ha]  | T-moves | 0.014375(6)      | 0.015376(8)  | 0.01560(2)       | 0.01673(2)   | 0.01313(1)   | 0.00341(3) |
| $\epsilon$ [mHa] | T-moves | 100.6(3)         | 114.8(3)     | 116.4(4)         | 141.7(6)     | 57.4(4)      | 1.6(1)     |
| $\eta$ [%]       | T-moves | 11.89(4)         | 12.14(3)     | 11.35(4)         | 11.18(5)     | 8.89(6)      | 2.3(1)     |

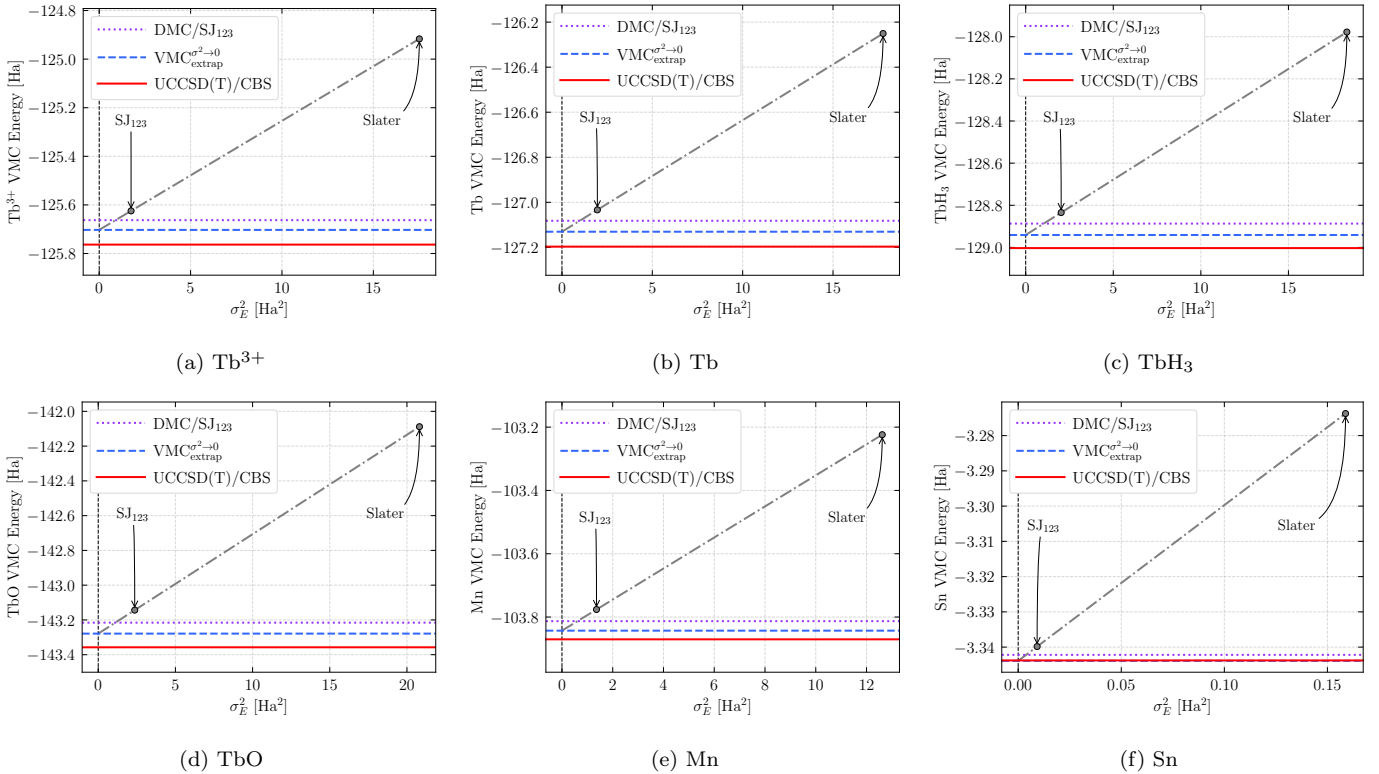

Supplementary Figure 14: VMC energy vs. variance extrapolations for molecular systems relevant for  $\text{TbMn}_6\text{Sn}_6$  using two data points: HF Slater and HF Slater+ $J_{123}$ .

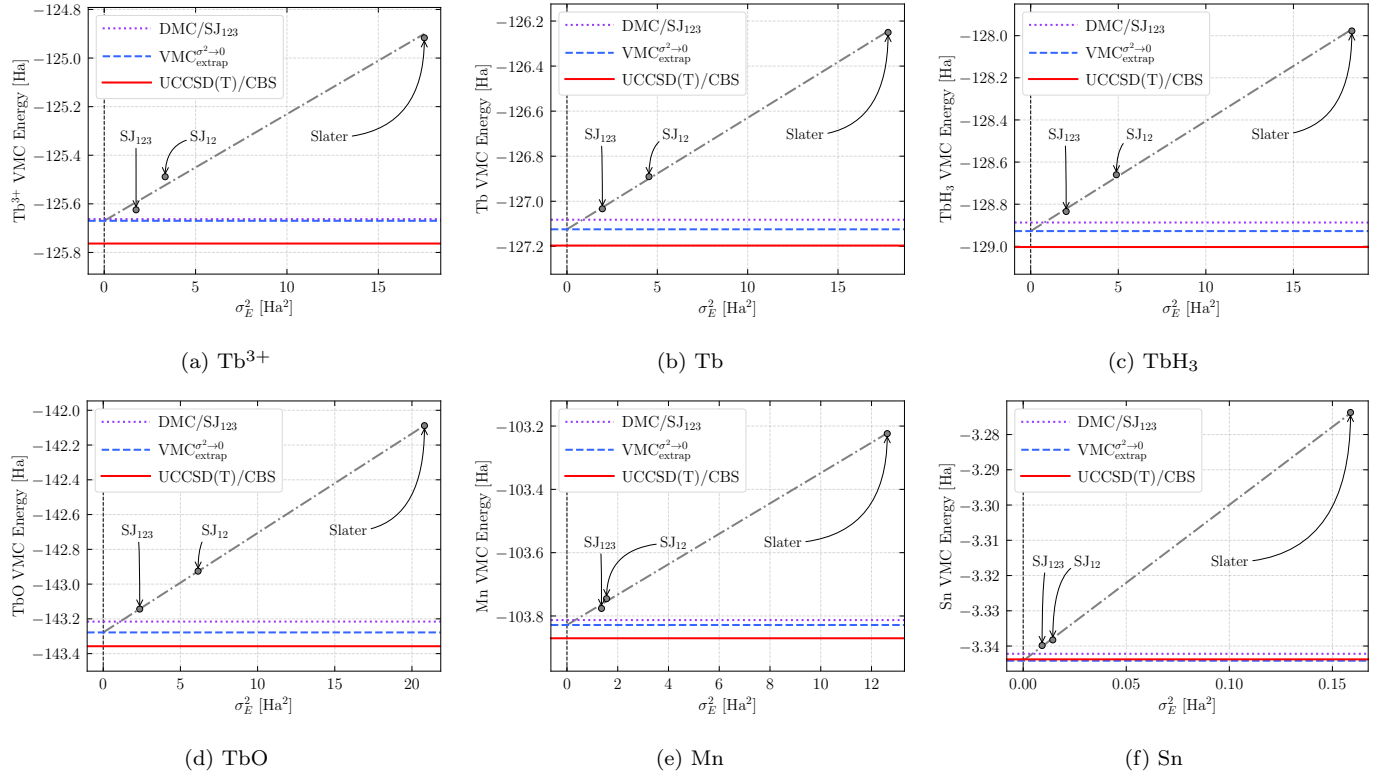

Supplementary Figure 15: VMC energy vs. variance extrapolations for molecular systems relevant for  $\text{TbMn}_6\text{Sn}_6$  using three data points: HF Slater, HF Slater+J<sub>12</sub>, and HF Slater+J<sub>123</sub>.

# SUPPLEMENTARY NOTE 5. DFT+EDMFT METHODS AND DATA

We use the embedded implementation of the all-electron density functional theory (DFT)+embedded-dynamical mean-field theory (DMFT) or DFT+eDMFT method. Here, the non-perturbative form of such self-energy is obtained by solving the quantum impurity problem in the presence of a self-consistent mean-field environment, where the self-energy is approximated by a quantity local to the atom in the unit cell. This work uses the fully self-consistent DFT+eDMFT implementation, where the quantum impurity method is solved by the continuous-time quantum Monte Carlo method, developed at Rutgers by Haule *et al.* [24]. The self-energy of the Mn  $d$ -orbital is embedded by the Dyson equation into the Hilbert space of all electrons in the solid using the projection/embedding technique [24]. This projection step connects the atomic degrees of freedom with the continuum degrees of freedom of the solid and leads to causal DMFT equations, which can capture the spectral weight of all electrons in the solid. Unlike the DFT method, DFT+eDMFT can address the excited state properties, as it is based on the Klein functional, in which the single-particle Green's function describes quasiparticle excitations of the solid and is not an auxiliary object. This approach is a minimal theory that is able to reconcile the itinerant and localized character of the electron, treating Hubbard bands and quasiparticle bands on the same footing. In the DFT+eDMFT method [24], we use the combination of DMFT and the LDA functional in the LAPW basis set as implemented in WIEN2k [25], where all higher-order Feynman diagrams are explicitly calculated by the impurity solver. This DFT+eDMFT implementation allows one to write down the total energy in terms of the stationary form of the energy functional. This implementation uses projectors for the very localized orbitals contained within the muffin-tin spheres. The projection is done on correlated  $d$ -orbitals within the Fermi energy  $\pm 10$  eV. The purpose of the projection is to extract the local Green's function from the full Green's function. Using the *exact* double-counting between LDA and eDMFT [26], the self-energy on Matsubara frequency is obtained. Then, it is analytically continued with the maximum entropy method from the imaginary to the real axis, continuing the local cumulant function to obtain the partial density of states and the spectral functions. A fine  $k$ -point mesh of at least  $12 \times 12 \times 6$   $k$ -points in Monkhorst-Pack  $k$ -point grid and a minimum of a total of 20 million Monte Carlo steps for each iteration are used for all the calculations, which are performed at  $T = 112$  K. Coulomb interaction  $U$  and Hund's coupling  $J_H$  are fixed at 5.0 eV and 0.8 eV, respectively, which is consistent with the constrained-DMFT calculation [27]. Supplementary Figure 16 shows the histogram plots for Mn  $3d$  orbital occupation  $N$  and fluctuating spin-states  $|S_z|$  in the paramagnetic phase of  $\text{TbMn}_6\text{Sn}_6$ . See the main text for discussions.

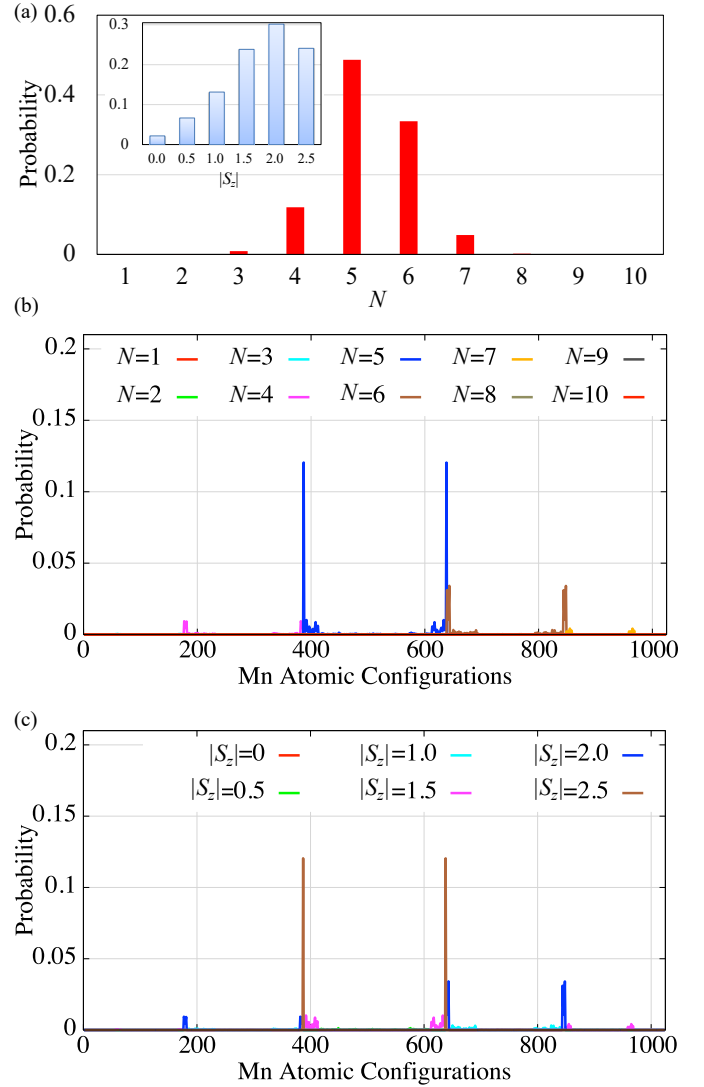

Supplementary Figure 16: DFT+eDMFT computed atomic histogram of the Mn  $3d$  shell in  $\text{TbMn}_6\text{Sn}_6$ . (a) Decomposed probability in the number of particles  $N$  and (inset) spin-state ( $|S_z|$ ). The probability distribution for all  $2^{10}$  (=1024) atomic configurations is shown for each (b)  $N$  and (c) spin state  $|S_z|$ .  $N$  and  $|S_z|$  values are denoted with various colors.

- 
- [1] B. C. El Idrissi, G. Venturini, B. Malaman, and D. Fruchart, Magnetic structures of  $\text{TbMn}_6\text{Sn}_6$  and  $\text{HoMn}_6\text{Sn}_6$  compounds from neutron diffraction study, *J. less-common met.* **175**, 143 (1991).
- [2] P. J. Hay and W. R. Wadt, Ab initio effective core potentials for molecular calculations. Potentials for K to Au including the outermost core orbitals, *J. Chem. Phys.* **82**, 299 (1988).
- [3] H. Stoll, B. Metz, and M. Dolg, Relativistic energy-consistent pseudopotentials—Recent developments, *J. Comput. Chem.* **23**, 767 (2002).
- [4] A. Bergner, M. Dolg, W. Küchle, H. Stoll, and H. Preuß, Ab initio energy-adjusted pseudopotentials for elements of groups 13–17, *Mol. Phys.* **80**, 1431 (1993).
- [5] G. Igel-Mann, H. Stoll, and H. Preuss, Pseudopotentials for main group elements (IIIa through VIIa), *Mol. Phys.* **65**, 1321 (1988).
- [6] M. Burkatzki, C. Filippi, and M. Dolg, Energy-consistent pseudopotentials for quantum Monte Carlo calculations, *J. Chem. Phys.* **126**, 234105 (2007).
- [7] J. R. Trail and R. J. Needs, Smooth relativistic Hartree–Fock pseudopotentials for H to Ba and Lu to Hg, *J. Chem. Phys.* **122**, 174109 (2005).
- [8] J. R. Trail and R. J. Needs, Norm-conserving Hartree–Fock pseudopotentials and their asymptotic behavior, *J. Chem. Phys.* **122**, 014112 (2005).
- [9] L. A. LaJohn, P. A. Christiansen, R. B. Ross, T. Atashroo, and W. C. Ermler, Ab initio relativistic effective potentials with spin–orbit operators. III. Rb through Xe, *J. Chem. Phys.* **87**, 2812 (1987).
- [10] W. J. Stevens, M. Krauss, H. Basch, and P. G. Jasien, Relativistic compact effective potentials and efficient, shared-exponent basis sets for the third-, fourth-, and fifth-row atoms, *Can. J. Chemistry* **70**, 612 (1992).
- [11] G. Wang, A. Annaberdiyev, C. A. Melton, M. C. Bennett, L. Shulenburger, and L. Mitas, A new generation of effective core potentials from correlated calculations: 4s and 4p main group elements and first row additions, *J. Chem. Phys.* **151**, 144110 (2019).
- [12] Pseudopotential Library: A community website for pseudopotentials/effective core potentials developed for high accuracy correlated many-body methods such as quantum Monte Carlo and quantum chemistry, <https://pseudopotentiallibrary.org> (2022), accessed: 2022-11-18.
- [13] A. Annaberdiyev, G. Wang, C. A. Melton, M. C. Bennett, L. Shulenburger, and L. Mitas, A new generation of effective core potentials from correlated calculations: 3d transition metal series, *J. Chem. Phys.* **149**, 134108 (2018).
- [14] J.-X. Yin, W. Ma, T. A. Cochran, X. Xu, S. S. Zhang, H.-J. Tien, N. Shumiya, G. Cheng, K. Jiang, B. Lian, Z. Song, G. Chang, I. Belopolski, D. Multer, M. Litskevich, Z.-J. Cheng, X. P. Yang, B. Swidler, H. Zhou, H. Lin, T. Neupert, Z. Wang, N. Yao, T.-R. Chang, S. Jia, and M. Zahid Hasan, Quantum-limit Chern topological magnetism in  $\text{TbMn}_6\text{Sn}_6$ , *Nat* **583**, 533 (2020).
- [15] G. Venturini, B. E. Idrissi, and B. Malaman, Magnetic properties of  $\text{RMn}_6\text{Sn}_6$  ( $\text{R} = \text{Sc}, \text{Y}, \text{Gd-Tm}, \text{Lu}$ ) compounds with  $\text{HfFe}_6\text{Ge}_6$  type structure, *J. Magn. Magn. Mater.* **94**, 35 (1991).
- [16] D. M. Clatterbuck and K. A. Gschneidner, Magnetic properties of  $\text{RMn}_6\text{Sn}_6$  ( $\text{R}=\text{Tb}, \text{Ho}, \text{Er}, \text{Tm}, \text{Lu}$ ) single crystals, *J. Magn. Magn. Mater.* **207**, 78 (1999).
- [17] C. Mielke III, W. L. Ma, V. Pomjakushin, O. Zaharko, S. Sturniolo, X. Liu, V. Ukleev, J. S. White, J.-X. Yin, S. S. Tsirkin, C. B. Larsen, T. A. Cochran, M. Medarde, V. Porée, D. Das, R. Gupta, C. N. Wang, J. Chang, Z. Q. Wang, R. Khasanov, T. Neupert, A. Amato, L. Liborio, S. Jia, M. Z. Hasan, H. Luetkens, and Z. Guguchia, Low-temperature magnetic crossover in the topological kagome magnet  $\text{TbMn}_6\text{Sn}_6$ , *Commun. Phys.* **5**, 1 (2022).
- [18] S. Kimura, A. Matsuo, S. Yoshii, K. Kindo, L. Zhang, E. Brück, K. Buschow, F. de Boer, C. Lefèvre, and G. Venturini, High-field magnetization of  $\text{RMn}_6\text{Sn}_6$  compounds with  $\text{R}=\text{Gd}, \text{Tb}, \text{Dy}$  and  $\text{Ho}$ , *J. Alloy. Compd.* **408–412**, 169 (2006).
- [19] D. C. Jones, S. Das, H. Bhandari, X. Liu, P. Siegfried, M. P. Ghimire, S. S. Tsirkin, I. I. Mazin, and N. J. Ghimire, Origin of Spin Reorientation and Intrinsic Anomalous Hall Effect in the Kagome Ferrimagnet  $\text{TbMn}_6\text{Sn}_6$ , Preprint at <https://arxiv.org/abs/2203.17246> (2022).
- [20] Y. Lee, R. Skomski, X. Wang, P. P. Orth, Y. Ren, B. Kang, A. K. Pathak, A. Kutepov, B. N. Harmon, R. J. McQueeney, I. I. Mazin, and L. Ke, Interplay between magnetism and band topology in the kagome magnets  $\text{RMn}_6\text{Sn}_6$ , *Phys. Rev. B* **108**, 045132 (2023).
- [21] M. Casula, Beyond the locality approximation in the standard diffusion Monte Carlo method, *Phys. Rev. B* **74**, 161102 (2006).
- [22] A. Annaberdiyev, C. A. Melton, M. C. Bennett, G. Wang, and L. Mitas, Accurate Atomic Correlation and Total Energies for Correlation Consistent Effective Core Potentials, *J. Chem. Theory Comput.* **16**, 1482 (2020).
- [23] L. Mitáš, E. L. Shirley, and D. M. Ceperley, Nonlocal pseudopotentials and diffusion Monte Carlo, *J. Chem. Phys.* **95**, 3467 (1991).
- [24] K. Haule, C.-H. Yee, and K. Kim, Dynamical mean-field theory within the full-potential methods: Electronic structure of  $\text{CeIrIn}_5$ ,  $\text{CeCoIn}_5$ , and  $\text{CeRhIn}_5$ , *Phys. Rev. B* **81**, 195107 (2010).
- [25] P. Blaha, K. Schwarz, G. K. H. Madsen, D. Kvasnicka, J. Luitz, R. Laskowski, F. Tran, L. Marks, and L. Marks, *WIEN2k: An Augmented Plane Wave Plus Local Orbitals Program for Calculating Crystal Properties* (Techn. Universität, 2019).
- [26] K. Haule, Exact double counting in combining the dynamical mean field theory and the density functional theory, *Phys. Rev. Lett.* **115**, 196403 (2015).
- [27] S. Mandal, K. Haule, K. M. Rabe, and D. Vanderbilt, Electronic correlation in nearly free electron metals with beyond-dft methods, *npj Comput. Mater.* **8**, 181 (2022).
